# Supplementary material for: Function on Scalar Regression with Complex Survey Designs
Source: arXiv:2511.05487 source file (2026-10-06)
Supplement: Supplementary file 1 [file Web_Appendix_A.pdf]

# Web Appendix A: Fast univariate inference for single level FoSR

## 1. BACKGROUND

Fast Univariate Inference (FUI) for single level function on scalar regression is outlined as a "scalable approach" in Chapter 5 of [1] and is a special case of the FUI approach for longitudinal functional data [2]. The approach consists of three steps: (1) fitting massively univariate generalized linear regression models at each point along the functional domain, (2) applying a smoothing procedure along the functional domain, and (3) constructing pointwise and joint confidence bands using analytic methods for Gaussian data or a bootstrap-based approach for non-Gaussian data. These steps are conceptually similar to those used in FUI for longitudinal functional data, but are specifically adapted for single level datasets where repeated measure are not present. Here we describe the three steps and perform simulations to demonstrate the method's performance under various settings.

## 2. UNIVARIATE FUNCTIONAL MODEL

Suppose the functional response for subject $i$ is of the type $Y_i(s)$ on a functional domain $\mathcal{L}$ for $\{s_1, s_2, \ldots, s_L\}$. $i = 1, \ldots, I$ is the index of the subject and $Y_i(s)$ may be Gaussian or non-Gaussian. We are interested in modeling the functional outcome $Y$ as a function of $p$ covariates, which we denote $\mathbf{X}_i = [X_{i1}, X_{i2}, \ldots, X_{ip}]^T$. The univariate functional approach is as follows:

1. At every point along the functional domain $s_l \in \mathcal{L}$, fit a pointwise generalized linear model:

$$\eta_i(s_l) = g(\mu_i(s_l)) = \beta_0 + X_i^T \beta$$

   Where $g(.)$ is a link function and $\mu_i(s_l)$ is the conditional mean $\mathbb{E}([Y_i(s_l)|X_i])$. From these regressions we obtain coefficient estimates at each point along the functional domain $\{\tilde{\mathbf{fi}}(s), s \in \mathcal{L}\}$

2. Smooth the coefficients $\tilde{\beta}$ along the functional domain with any type of smoother. Denote smooth estimators as $\{\hat{\beta}(s), s \in \mathcal{L}\}$

3. Calculate joint and pointwise confidence bands for the coefficient estimates via bootstrap or analytic approaches.

## 3. INFERENCE

We use the same approach as [2] - bootstrapping participants - in the bootstrap-based approach for inference. The procedure is as follows for $B$ bootstrap repetitions.
**Data**: $\{\mathbf{Y}(s_l), l \in \mathcal{L}\}, \mathbf{X}$
**Result**: $Var(\boldsymbol{\beta}(s_l)), l \in \mathcal{L}$
for $b = 1, \ldots, B$, **do:**

1. Obtain a vector of resampled indices $D_{(b)}$ by sampling with replacement indices from $1, \ldots, I$.

2. The $bth$ bootstrap sample is thus $\{\{\mathbf{Y}_{D_{(b)}}(s_l), l \in \mathcal{L}\}, \mathbf{X}_{D_{(b)}}\}$

3. Fit the model from section xx using the $bth$ bootstrap sample. Obtain the coefficient estimates $\{\boldsymbol{\beta}(s_l)_{(b)}, l \in \mathcal{L}\}$
   **end**

4. For $l \in \mathcal{L}$, estimate $Var(\boldsymbol{\beta}(s_l))$ from the $B$ bootstrap estimates

## 4. CONFIDENCE BANDS

To derive joint confidence bands, we follow the same approach outlined in section 4 of [2] of simulating from the multivariate normal distribution using a PCA decomposition of bootstrap samples.

## 5. SIMULATIONS

The goal of the simulations are to evaluate the accuracy of the estimators and the performance of pointwise and joint confidence intervals, and compare the method to existing approaches for function on scalar regression.

### A. Setup

We use the following data generating model:

$$\eta_i(s) = g\{\mu_i(s)\} = \beta_0(s) + X_{i1}\beta_1(s), s \in \mathcal{L}$$

Where:
$X_{i1} \sim \mathcal{N}(0, 2^2)$. We vary the following components of the simulation:

1. Parameters

- Distribution of response
  - Gaussian: $g(x) = x$,
  $$Y_i(s) \sim \mathcal{N}(\mu_i(s) + \epsilon_i), \epsilon_i \sim \mathcal{N}(0, \sigma^2)$$
  - Binary: $g(x) = \frac{\exp(x)}{1+\exp(x)}$,
  $$Y_i(s) \sim Bernoulli(p = \eta_i(s))$$
  - Count: $g(x) = \exp(x)$,
  $$Y_i(s) \sim Poisson(\lambda = \eta_i(s))$$
- Functional coefficients $\boldsymbol{\beta}(s)$
  - S1: $\beta_0(s) = -0.15 - 0.1 * \sin(2\pi s) - 0.1 * \cos(2\pi s); \beta_1(s) = \frac{1}{20}(\frac{s-0.6}{0.0225})$
  - S2: $\beta_0(s) = 0.53 + 0.06\sin(3\pi s) - 0.03\sin(6.5\pi s); \beta_1(s) = \frac{1}{60}\phi(\frac{s-0.2}{0.1^2} + \frac{1}{200}\phi(\frac{s-0.35}{0.1^2}) - \frac{1}{250}\phi(\frac{s-0.65}{0.06^2}) + \frac{1}{60}\phi(\frac{s-1}{0.07^2})$
- Sample size
  - Number of observations: $I \in \{100, 500, 1000, 10{,}000\}$
  - Dimension of functional domain: $\mathcal{L} \in \{50, 100, 500\}$
- Signal to noise ratio (SNR) (only for Gaussian data)
  - SNR $\in \{0.5, 1, 5\}$

### B. Code

R code for FUI can be found at https://github.com/jhuwit/survey_FoSR. The code used to fit the FAMM is as follows:

### C. Comparison to existing methods

We compare this method to function on scalar regression with penalized basis expansions [3]. We use `refund::pffr` with `algorithm = "bam"` and `method="fREML"` to speed up computation. We use 15 and 20 cubic B-splines bases with first order difference penalty for the population average and global functional intercept, respectively ( `bs.yindex = list(bs = "ps", k = 15, m = c(2, 1))`, `bs.int = list(bs = "ps", k = 20, m = c(2, 1))`).

```
fit_pffr =
        sample_data %>%
        select(-starts_with("Y")) %>%
        mutate(Y_mat = I(Y_mat)) %>%
        refund::pffr(
          Y_mat ~ X,
          data = .,
          algorithm = "bam",
          family = temp$family,
          method = "fREML",
          bs.yindex = list(
            bs = "ps",
            k = 15,
            m = c(2, 1)
          )
        )
```

### D. Evaluation criteria

We use two criteria to compare the models: (1) accuracy in coefficient estimation and (2) inference of coefficient estimation. To address (1): integrated square error is calculated for each coefficient and simulation, defined as $ISE_k = \int_{\mathcal{L}} (\hat{\beta}_k(l) - \beta_k(l) dl, k = 0, 1$. Mean integrated square error is calculated by taking the average ISE across all simulation iterations. Inference for coefficient estimation is assessed by computing the average of the pointwise coverage probability across the functional domain from the 95% confidence bands. For each simulation scenario, we do 200 simulations. For bootstrap, we use 500 bootstrap repetitions.

### E. Simulation results

The full simulation results can be found at https://github.com/jhuwit/survey_FoSR/blob/main/results/simulations/all_nonsurvey_sim_res.rds.

**Accuracy** The baseline setting is SNR = 1, $n = 500$, $L = 100$, and scenario = 1. For all plots, the baseline settings are kept constant for all except one parameter of the simulation.

1. Signal to noise parameters
   The log base 10 mean integrated squared error (MISE) for gaussian data at different signal to noise ratios and for each scenario are shown in the top panel of Figure S1. Bias is similar between FAMM and FUI with the exception of high SNR and scenario 2, where FUI has much lower bias. The lower panel of Figure S1 displays the bias for each scenario in for Bernoulli (left) and Poisson (right) data. Bias is similar between FAMM and FUI.

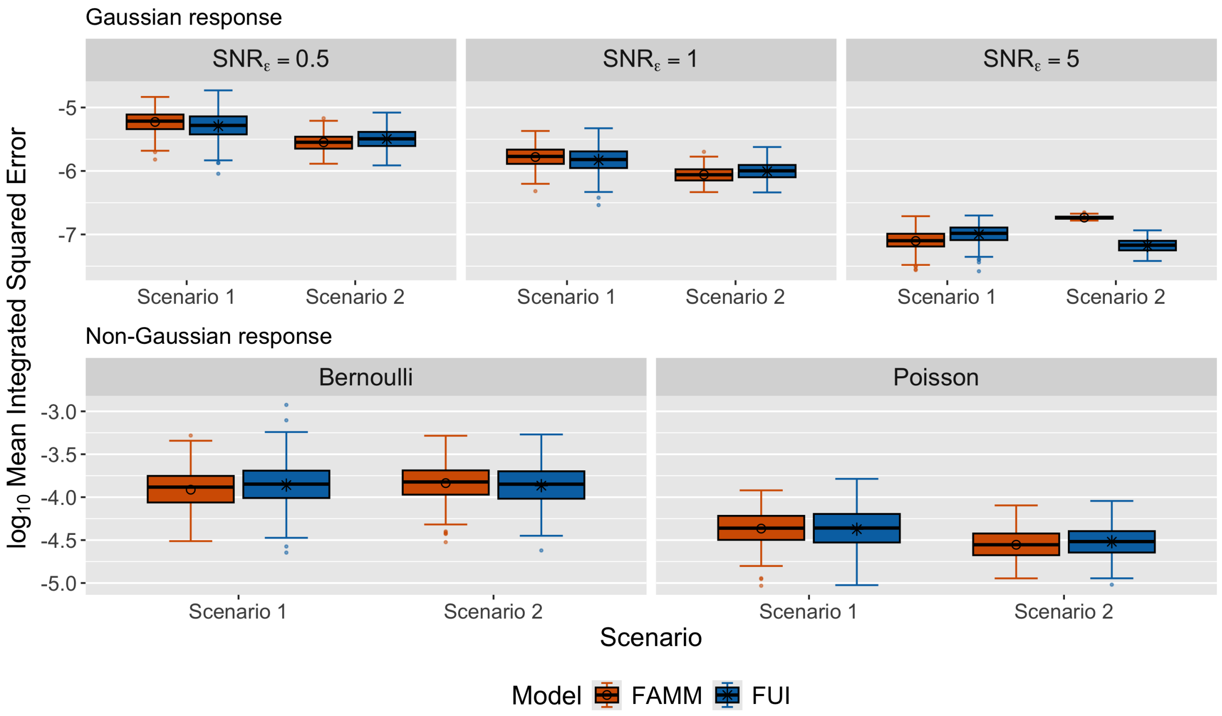


**Fig. S1.** Log Mean Integrated Squared Error (MISE) for gaussian data at different noise levels (top panel) and Bernoulli and Poisson data (bottom panel). For all plots, $n$ is fixed at 500 and $L$ at 100.

2. Sample size parameters
   Log 10 MISE for gaussian data at varying sample sizes with fixed $L$ is shown in the top panel of Figure S2, while log MISE for gaussian data at varying functional domain lengths with fixed $n$ is shown in the bottom panel. Bias for FUI and FAMM is similar, although bias tends to be higher for FAMM scenario 2 at large sample sizes. Bias was similar between FAMM and FUI for Poisson data (see Figure S3) and Bernoulli data (see Figure S4).

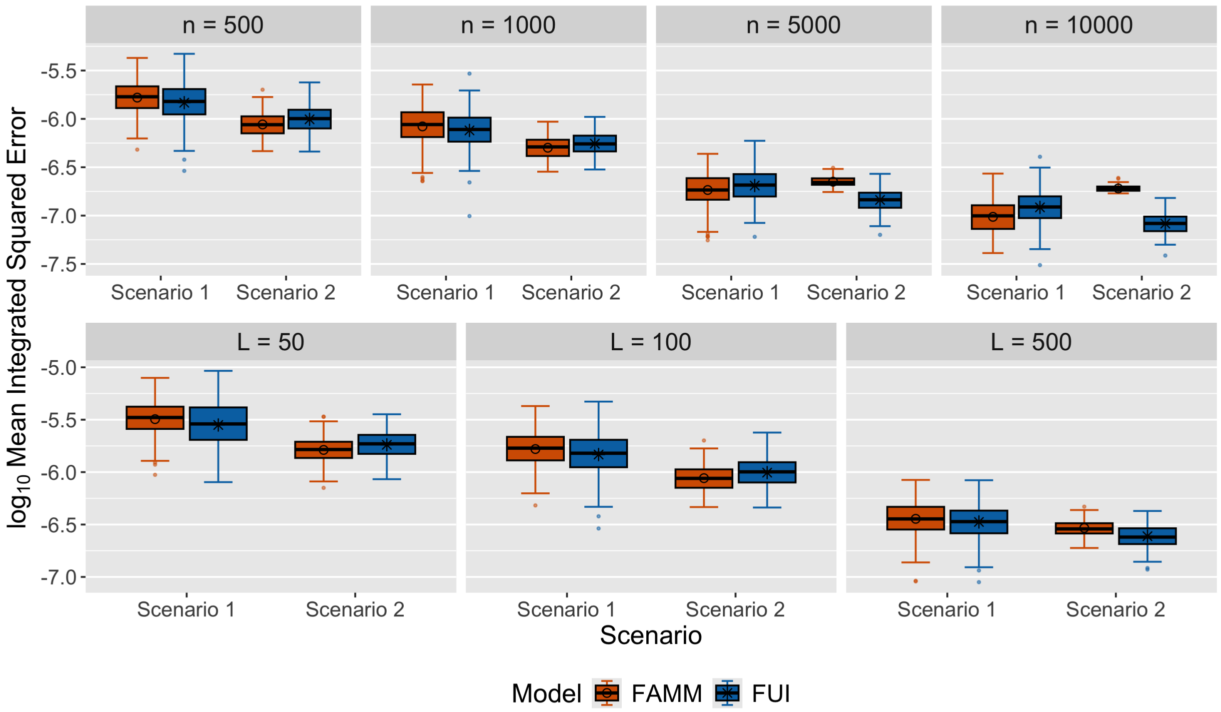


**Fig. S2.** Log 10 Mean Integrated Squared Error (MISE) for Gaussian data across different sample sizes when $L = 100$ (top panel) and different lengths of the functional domain when $n = 500$ (bottom panel). For all plots, SNR is fixed at 1.

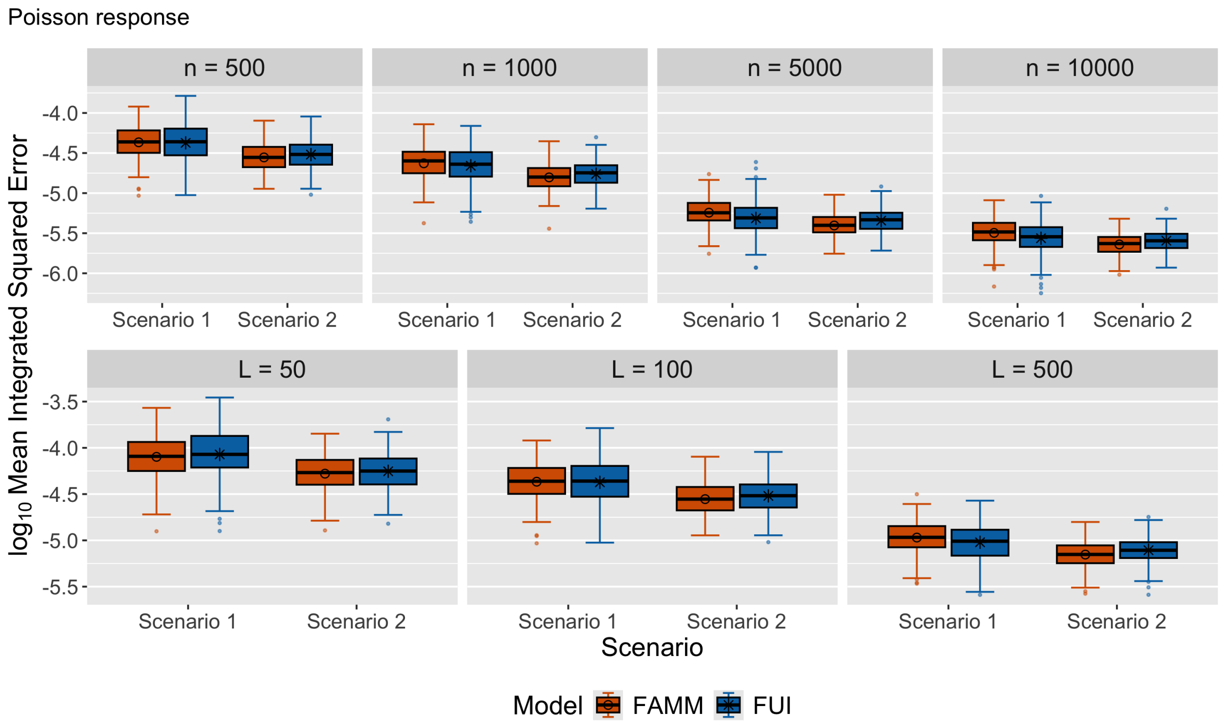


**Fig. S3.** Log Mean Integrated Squared Error (MISE) for Poisson data across different sample sizes when $L = 100$ (top panel) and different lengths of the functional domain when $n = 500$ (bottom panel).

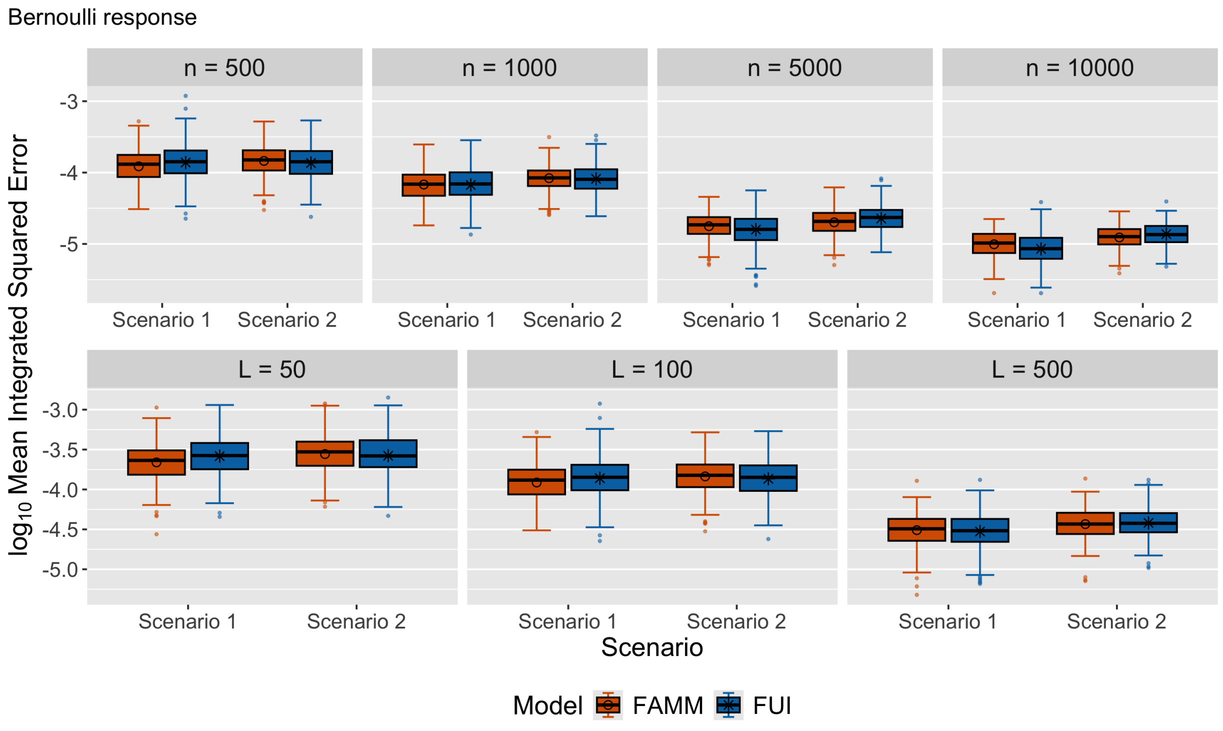


**Fig. S4.** Log Mean Integrated Squared Error (MISE) for Bernoulli data across different sample sizes when $L = 100$ (top panel) and different lengths of the functional domain when $n = 500$ (bottom panel).

**Inference**
Table S1 displays mean coverage rates for different simulation settings. Both FAMM and FUI achieve the 95% pointwise coverage rate for all settings and FUI achieves the joint coverage rate of 95% as well.

| $L = 100$, SNR = 1, Gaussian | | **n=500** | | **n=10000** | | **n=5000** | | **n=1000** | |
|---|---|---|---|---|---|---|---|---|---|
| | | S1 | S2 | S1 | S2 | S1 | S2 | S1 | S2 |
| FAMM | Pointwise coverage | 0.96 | **0.90** | 0.95 | **0.87** | 0.95 | **0.69** | 0.95 | **0.56** |
| FUI | Pointwise coverage | 0.96 | 0.95 | 0.96 | 0.95 | 0.94 | 0.94 | 0.94 | 0.94 |
| FUI | Joint Coverage | 0.97 | **0.89** | 0.96 | **0.87** | **0.92** | **0.80** | **0.88** | **0.80** |
| $n = 500$, SNR = 1, Gaussian | | **L=50** | | **L=100** | | **L=500** | | | |
| | | S1 | S2 | S1 | S2 | S1 | S2 | | |
| FAMM | Pointwise coverage | 0.96 | **0.92** | 0.96 | **0.90** | 0.95 | **0.79** | | |
| FUI | Pointwise coverage | 0.95 | 0.95 | 0.96 | 0.95 | 0.96 | 0.95 | | |
| FUI | Joint Coverage | 0.97 | **0.89** | 0.97 | **0.89** | 0.94 | **0.70** | | |
| $L = 100, n = 500$, Gaussian | | $\textbf{SNR}_\epsilon = 0.5$ | | $\textbf{SNR}_\epsilon = 1$ | | $\textbf{SNR}_\epsilon = 5$ | | | |
| | | S1 | S2 | S1 | S2 | S1 | S2 | | |
| FAMM | Pointwise coverage | 0.96 | 0.93 | 0.96 | **0.90** | 0.95 | **0.53** | | |
| FUI | Pointwise coverage | 0.96 | 0.94 | 0.96 | 0.95 | 0.94 | 0.95 | | |
| FUI | Joint Coverage | 0.97 | **0.88** | 0.97 | **0.89** | **0.91** | **0.86** | | |
| $L = 100, n = 500$, SNR = 1 | | **Gaussian** | | **Bernoulli** | | **Poisson** | | | |
| | | S1 | S2 | S1 | S2 | S1 | S2 | | |
| FAMM | Pointwise coverage | 0.96 | **0.90** | 0.96 | 0.95 | 0.96 | 0.95 | | |
| FUI | Pointwise coverage | 0.96 | 0.95 | 0.95 | 0.96 | 0.96 | 0.93 | | |
| FUI | Joint Coverage | 0.97 | **0.89** | 0.94 | 0.96 | 0.97 | **0.83** | | |

**Table S1.** Mean coverage across different simulation settings for FAMM and FUI. Settings where coverage is less than 0.93 are bolded.

### F. Simulation summary

The FUI method for single-level functional data achieves similar accuracy to FAMM and meets the nominal coverage rate for 95% for both pointwise confidence intervals across a variety of data generating mechanisms, sample sizes, length of functional domain, signal to noise ratios, and data distributions.

## REFERENCES

1. C. Crainiceanu, J. Goldsmith, A. Leroux, and E. Cui, *Functional Data Analysis with R* (Springer New York, NY, USA, 2024).
2. E. Cui, A. Leroux, E. Smirnova, and C. M. Crainiceanu, “Fast Univariate Inference for Longitudinal Functional Models,” J. Comput. Graph. Stat. **31**, 219–230 (2021).
3. P. T. Reiss, L. Huang, and M. Mennes, “Fast Function-on-Scalar Regression with Penalized Basis Expansions,” The Int. J. Biostat. **6** (2010).
