# Supplementary material for: Function on Scalar Regression with Complex Survey Designs
Source: arXiv:2511.05487 source file (2026-10-06)
Supplement: Supplementary file 2 [file Web_Appendix_B.pdf]

# Web Appendix B: Simulation code

## 1. CODE FOR DATA GENERATION AND SAMPLING

```
I <- 10e6 # population size
num_strata <- 30
dirichlet_probs <- gtools::rdirichlet(1, rep(4, num_strata))
stratum_assignments <- sample(1:num_strata, I, replace = TRUE, prob = dirichlet_probs)
for (s in 1:num_strata) {
  set.seed(seed + s)
  num_in_strata = sum(stratum_assignments == s)
  num_psu = round(runif(1, 75, 125), 0)
  set.seed(seed + s)
  dps = gtools::rdirichlet(1, rep(10, num_psu))
  set.seed(seed + s)
  psu_in_stratum = sample(1:num_psu, num_in_strata, replace = TRUE, prob = dps)
}
set.seed(seed)
stratum_scaling <- rnorm(num_strata, mean = 1, sd = sd_beta)
beta1_by_stratum <- matrix(
    rep(stratum_scaling, each = L), nrow = num_strata, byrow = TRUE) *
    matrix(rep(beta_fixed[2, ], times = num_strata), nrow = num_strata, byrow = TRUE)
nbasis <- 5
basis <- fda::create.bspline.basis(c(0, 1), nbasis)
Phi <- fda::eval.basis(grid, basis)

set.seed(seed)
strata_scores <- matrix(rnorm(num_strata * nbasis, 0, strata_sigma), num_strata, nbasis)
strata_random_effects <- strata_scores %*% t(Phi)
total_psu = length(unique(psu_assignments))
set.seed(seed)
psu_scores <- matrix(rnorm(total_psu * nbasis, 0, psu_sigma), total_psu, nbasis)
psu_random_effects <- psu_scores %*% t(Phi)
strata_effects_indiv <- strata_random_effects[stratum_assignments, ]
psu_effects_indiv <- psu_random_effects[as.numeric(factor(psu_assignments)), ]
random_effects <- strata_effects_indiv + psu_effects_indiv
fixef_signal <- matrix(rep(beta_fixed[1, ], I), nrow = I, byrow = TRUE) +
    X_des[, 2] * matrix(rep(beta_fixed[2, ], I), nrow = I, byrow = TRUE)
  # include stratum-specific slope variation in the random effects
slope_re <- (stratum_scaling[stratum_assignments] - 1) *
matrix(rep(beta_fixed[2, ], I), nrow = I, byrow = TRUE)
ranef <- slope_re + random_effects
ranef <- sd(fixef_signal) / sd(ranef) / snr_b * ranef
get_p_i = function(i, probs) probs[i] * (1 + sum((probs[-i]) / (1-probs[-i])))

for (strata in 1:num_strata) {
    # strata = 1
    # individuals in the strata
    inds_in_stratum <- which(stratum_assignments == strata)
    # Get PSU sizes in this stratum
    psu_sizes <- table(psu_assignments[inds_in_stratum])
    psu_ids <- names(psu_sizes)
    # Sample PSUs without replacement using PPS
    set.seed(strata + seed)
    selected_psus <- sample(psu_ids, size = num_selected_psu, replace = FALSE,
    prob = psu_sizes)
    psu_probs <- psu_sizes / sum(psu_sizes)  # PPS
    psu_prob_selected = map_dbl(.x = match(selected_psus, psu_ids), .f = get_p_i, psu_probs)

    names(psu_prob_selected) <- selected_psus
    # within each selected PSU select individuals based on X1
```

```
    for (psu in selected_psus) {
      inds_in_psu <- which(psu_assignments == psu & stratum_assignments == strata)
    if (inf_level == 0) {
        # Uniform sampling
        n = length(inds_in_psu)
        inclusion_probs = rep(1 / n, n)
      } else {
        # Compute mean outcome in PSU
        y_mean = rowMeans(Y_obs[inds_in_psu, ])

        # Compute inclusion score depending on family
        incl_score = switch(family,
                             "gaussian" = y_mean * inf_level,
                             "poisson"  = log(y_mean) * inf_level,
                             "binomial" = qlogis(pmin(pmax(y_mean, 1e-6), 1e-6)) * inf_level,
                             stop("Unknown family"))

        # apply compression and map to probabilities
        score_compressed = pmax(pmin(incl_score, compression), -compression)
        inclusion_probs = plogis(score_compressed)
      }
      inclusion_probs_adj = inclusion_probs / sum(inclusion_probs) * I_n
      inclusion_probs_adj[inclusion_probs_adj > 1]  = 1
      # ensure reproducibility
      set.seed(strata + seed + which(selected_psus == psu))
      sampled_units = inds_in_psu[rbinom(length(inds_in_psu), 1, inclusion_probs_adj) == 1]
      final_sample = c(final_sample, sampled_units)
      psus = c(psus, rep(psu, length(sampled_units)))
      p_psu = psu_prob_selected[which(names(psu_prob_selected) == psu)]
      p1[inds_in_psu]  = p_psu
      p2[inds_in_psu]  = inclusion_probs_adj
      p_overall[inds_in_psu]  = p_psu * inclusion_probs_adj
    }
  }
```

## 2. FUNCTIONS FOR RUNNING SIMULATION

```
required_packages <- c("svrep", "purrr", "progress", "svylme", 'dplyr', 'readr', 'refund', 'gtools')

install_and_load <- function(package) {
  if (!require(package, character.only = TRUE)) {
    install.packages(package)
    library(package, character.only = TRUE)
  }
}

library(here)
library(devtools)
library(fastFMM)
library(haven)
library(dplyr)
library(survey)
library(progress)
library(lme4)
library(mgcv)
library(ggplot2)
library(gridExtra)
library(svrep)


# get beta hat
get_betatilde = function(data, family = "gaussian", type = "weighted",
                         model_formula = as.formula(paste0('Y~', 'X'))){
  if(!(type %in% c("weighted", "unweighted"))){
    stop("please specify boot_type as one of 'weighted', 'unweighted'")
  }
```

```r
  out_index <- grep(paste0("^", model_formula[2]), names(data)) # indices that start with the outcome name
  if(length(out_index) != 1){ # functional observations stored in multiple columns
    L <- length(out_index)
  }else{ # observations stored as a matrix in one column using the I() function
    L <- ncol(data[,out_index])
  }
  argvals <- 1:L

  unimm_wt <- function(l) {
    data$Yl <- unclass(data[, out_index][, l])

    fit_uni <- suppressMessages(
      glm(
        formula = stats::as.formula(paste0("Yl ~ ", model_formula[3])),
        family = family,
        control = glm.control(maxit = 5000),
        weights = weight,
        data = data
      )
    )
    betaTilde <- coef(fit_uni)
    return(list(betaTilde = betaTilde))
  }
  unimm <- function(l) {
    data$Yl <- unclass(data[, out_index][, l])
    fit_uni <- suppressMessages(glm(
      formula = stats::as.formula(paste0("Yl ~ ", model_formula[3])),
      family = family,
      control = glm.control(maxit = 5000),
      data = data
    ))
    betaTilde <- coef(fit_uni)
    return(list(betaTilde = betaTilde))
  }
  if (type == "weighted") {
    massmm <- lapply(argvals, unimm_wt)
  } else if (type == "unweighted") {
    massmm <- lapply(argvals, unimm)
  }

  # Obtain betaTilde, fixed effects estimates
  betaTilde <- t(do.call(rbind, lapply(massmm, '[[', 1)))
  colnames(betaTilde) <- argvals
  return(betaTilde)
}

get_betahat = function(betaTilde, L,
                       nknots_min = NULL){
  argvals = 1:L
  nknots <- if (is.null(nknots_min)) round(L / 2) else min(round(L / 2), nknots_min)


  betaHat <- t(apply(betaTilde, 1, function(x) mgcv::gam(x ~ s(argvals, bs = "tp",
                                                                k = (nknots + 1)),
                                                          method = "GCV.Cp")$fitted.values))
                                                        method = "GCV.Cp")$fitted.values))
  rownames(betaHat) <- rownames(betaTilde)
  colnames(betaHat) <- 1:L
  return(betaHat)
}


lm_wls_multi <- function(X, Y, w) {
  # X: (n × p), Y: (n × L), w: (n)
```

```
  W_half <- sqrt(w)
  Xw <- X * W_half
  Yw <- Y * W_half
  # Solve weighted least squares for all outcomes at once
  coef_mat <- qr.coef(qr(Xw), Yw)
  # returns (p × L) coefficient matrix
  coef_mat
}

lm_multi <- function(X, Y) {
  # X: (n × p), Y: (n × L)
  # Solve OLS for multiple outcomes at once
  coef_mat <- qr.coef(qr(X), Y)
  # returns (p × L) coefficient matrix
  coef_mat
}

glm_batch_multiY <- function(
    X, y_mat, w = NULL,
    family,
    add_intercept = TRUE,
    offset = NULL,               # length-n or n x B (broadcasted if needed)
    start = NULL,                # optional p[+1]-vector to warm start all columns
    maxit = 50, tol = 1e-8, ridge = 1e-8,
    return_se = TRUE, estimate_phi = TRUE, verbose = FALSE
) {
  stopifnot(is.matrix(X), is.matrix(y_mat))
  n <- nrow(X); p <- ncol(X); B <- ncol(y_mat)
  stopifnot(nrow(y_mat) == n)

  if (is.null(w)) {
    w <- rep(1, n)   # no weights → all equal to 1
  }
  stopifnot(length(w) == n, is.numeric(w))

  if (add_intercept) X <- cbind(Intercept = 1, X)
  p <- ncol(X)

  # offsets: allow NULL (zeros), length-n (shared), n x 1 (shared), or n x B (per column)
  if (is.null(offset)) {
    offset <- matrix(0, n, B)
  } else if (is.vector(offset) && length(offset) == n) {
    offset <- matrix(offset, n, B)
  } else if (is.matrix(offset) && nrow(offset) == n && ncol(offset) == 1) {
    offset <- matrix(offset[,1], n, B)
  } else if (is.matrix(offset) && nrow(offset) == n && ncol(offset) == B) {
    # as provided
  } else {
    stop("offset must be NULL, length-n, n×1, or n×B")
  }

  # family bits
  linkinv    <- family$linkinv
  mu_eta_fun <- family$mu.eta
  variance   <- family$variance
  dev_resids <- family$dev.resids

  eps <- .Machine$double.eps^(2/3)

  # warm start
  if (!is.null(start)) {
    stopifnot(length(start) == p)
    Beta <- matrix(start, p, B)
  } else {
    Beta <- matrix(0, p, B)
```

```
}

# Precompute X' once
Xt <- t(X)

converged <- rep(FALSE, B)
it <- 0L

for (it in seq_len(maxit)) {
  # ETA & MU (n x B)
  Eta <- X %*% Beta
  Eta <- Eta + offset
  Eta <- pmin(pmax(Eta, -35), 35)
  Mu  <- linkinv(Eta)

  # dmu/deta and Var(mu) (n x B)
  mu_eta <- mu_eta_fun(Eta); mu_eta[abs(mu_eta) < eps] <- eps
  VarMu  <- variance(Mu);    VarMu[VarMu  < eps] <- eps

  # IRLS working weights and responses
  # Ww = w * (dmu/deta)^2 / Var(mu)  (n x B), z = eta + (y - mu) / (dmu/deta)
  Ww <- (mu_eta^2 / VarMu)
  Ww <- Ww * matrix(w, n, B)      # broadcast w across columns
  Z  <- Eta + (y_mat - Mu) / mu_eta

  # RHS for all fits at once: X' (Ww * Z)  (p x B)
  RHS <- Xt %*% (Ww * Z)

  step_max <- rep(0, B)
  active <- which(!converged)
  if (!length(active)) break

  # For each column, H_b = X' diag(w * s_b) X where s_b = (dmu/deta)^2 / Var(mu)
  s_all <- (mu_eta^2 / VarMu)      # n x B (without prior weights)
  for (b in active) {
    wb <- w * s_all[, b]            # length-n
    if (!any(is.finite(wb)) || sum(wb) < eps) next

    # Efficient: crossprod(X, wb * X) without forming diag
    Xw <- X * wb
    H  <- Xt %*% Xw
    diag(H) <- diag(H) + ridge

    beta_new <- tryCatch({
      Rchol <- chol(H)
      backsolve(Rchol, forwardsolve(t(Rchol), RHS[, b]))
    }, error = function(e) solve(H, RHS[, b], tol = 1e-12))

    step_max[b] <- max(abs(beta_new - Beta[, b]))
    Beta[, b]   <- beta_new
  }

  newly_conv <- (!converged) & (step_max < tol)
  converged[newly_conv] <- TRUE

  if (verbose) {
    cat(sprintf("Iter %d: active=%d, max step=%.3e\n",
                it, length(active), if (length(active)) max(step_max[active]) else 0))
  }
  if (all(converged)) break
}

out <- list(coef = Beta, iter = it, converged = converged)

if (return_se) {
```

```r
    # recompute at solution
    Eta <- X %*% Beta + offset
    Eta <- pmin(pmax(Eta, -35), 35)
    Mu  <- linkinv(Eta)
    mu_eta <- mu_eta_fun(Eta); mu_eta[abs(mu_eta) < eps] <- eps
    VarMu  <- variance(Mu);    VarMu[VarMu  < eps] <- eps
    s_all  <- (mu_eta^2 / VarMu)

    # dispersion (phi) per column if needed
    fam_name <- tolower(family$family)
    phi <- rep(1, B)
    needs_phi <- estimate_phi && !grepl("binomial|poisson", fam_name)
    if (needs_phi) {
      for (b in seq_len(B)) {
        wb <- w
        wb[!is.finite(wb) | wb < 0] <- 0
        phi[b] <- sum(dev_resids(y_mat[, b], Mu[, b], wb)) / max(n - p, 1L)
      }
    }

    SE <- matrix(NA_real_, p, B, dimnames = list(colnames(X), colnames(y_mat)))
    vcov_list <- vector("list", B)
    for (b in seq_len(B)) {
      wb <- w * s_all[, b]
      if (!any(is.finite(wb)) || sum(wb) < eps) next
      H <- Xt %*% (X * wb)
      diag(H) <- diag(H) + ridge
      invH <- tryCatch({
        Rchol <- chol(H); chol2inv(Rchol)
      }, error = function(e) solve(H, tol = 1e-12))
      vc <- invH * phi[b]
      vcov_list[[b]] <- vc
      SE[, b] <- sqrt(pmax(diag(vc), 0))
    }
    out$se <- SE
    out$vcov <- vcov_list
    out$phi <- phi
  }

  out
}


run_boots_xfast = function(data, boot_type, betaHat, family = "gaussian",
                           num_boots = 500, seed = 2025, L,
                           samp_stages = NULL,
                           model_formula = as.formula(paste0('Y~', 'X'))) {
  if(!(boot_type %in% c("BRR", "Rao-Wu-Yue-Beaumont", "weighted", "unweighted"))){
    stop("please specify boot_type as one of 'BRR', 'Rao-Wu-Yue-Beaumont', 'weighted', 'unweighted'")
  }
  argvals = 1:L
  data = data %>%
    mutate(row_id = row_number())
  out_index <- grep(paste0("^", model_formula[2]), names(data))
  Y_mat <- as.matrix(data[, out_index])
  X_base <- model.matrix(stats::as.formula(paste0("~", model_formula[3])), data = data)

  if (is.character(family)) {
    family <- get(family, mode = "function", envir = parent.frame())()
  }
  if (boot_type == "BRR") {
    sample_data = function(df) {
      df %>%
        group_by(strata) %>%
        summarise(psu = sample(psu, size = 1))
```

```
    }
    set.seed(seed)
    indices = replicate(num_boots, sample_data(data), simplify = FALSE)
  } else if (boot_type == "weighted") {
    set.seed(seed)
    boot_indices <- replicate(
      num_boots,
      sample(
        seq_len(nrow(data)),
        size = nrow(data),
        replace = TRUE,
        prob = data$weight / sum(data$weight)
      ),
      simplify = FALSE
    )
  } else if (boot_type == "unweighted") {
    set.seed(seed)
    boot_indices <- replicate(num_boots,
                              sample(
                                seq_len(nrow(data)),
                                size = nrow(data),
                                replace = TRUE
                              ),
                              simplify = FALSE)
    # boot_indices2 = matrix(sample(1:nrow(data), size = num_boots * nrow(data), replace = TRUE),
    #                        ncol = num_boots)
  }
  if (boot_type == "BRR") {
    # Weighted least squares for Gaussian case
    coefs = lapply(1:num_boots, function(r) {
      dat_tmp = data %>%
        inner_join(indices[[r]], by = c("psu", "strata")) %>%
        mutate(weight = weight * 2)

      X_tmp = X_base[dat_tmp$row_id, , drop = FALSE]
      Y_tmp = Y_mat[dat_tmp$row_id, , drop = FALSE]  # all L outcomes

      if (family$family == "gaussian") {
        # Fit all L responses at once
        coef_mat = lm_wls_multi(X_tmp, Y_tmp, dat_tmp$weight)
      } else {
        coef_mat = glm_batch_multiY(X = X_tmp, y_mat = Y_tmp, w = dat_tmp$weight, family = family,
        return_se = FALSE, add_intercept = FALSE)$coef
      }
      coef_mat  # (p × L)
    })

    # Convert list of matrices → array (p × L × num_boots)
    betaTilde_boot = simplify2array(coefs)
  } else if (boot_type == "unweighted") {
    coefs = lapply(1:num_boots, function(r) {
      dat_tmp <- data[boot_indices[[r]], ]
      X_tmp = X_base[dat_tmp$row_id, , drop = FALSE]
      Y_tmp = Y_mat[dat_tmp$row_id, , drop = FALSE]  # all L outcomes

      if (family$family == "gaussian") {
        # Fit all L responses at once
        coef_mat = lm_multi(X_tmp, Y_tmp)
      } else {
        coef_mat = glm_batch_multiY(X = X_tmp, y_mat = Y_tmp, family = family,
        return_se = FALSE, add_intercept = FALSE)$coef
      }
      coef_mat  # (p × L)
    })
    betaTilde_boot = simplify2array(coefs)
```

```
  } else if (boot_type == "weighted") {
    coefs = lapply(1:num_boots, function(r) {
      dat_tmp <- data[boot_indices[[r]], ]
      X_tmp = X_base[dat_tmp$row_id, , drop = FALSE]
      Y_tmp = Y_mat[dat_tmp$row_id, , drop = FALSE]  # all L outcomes
      if (family$family == "gaussian") {
        # Fit all L responses at once
        coef_mat = lm_wls_multi(X_tmp, Y_tmp, dat_tmp$weight)
      } else {
        coef_mat = glm_batch_multiY(X = X_tmp, y_mat = Y_tmp, w = dat_tmp$weight, family = family,
        return_se = FALSE,add_intercept = FALSE)$coef
      }
      coef_mat  # (p × L)
    })
    # Convert list of matrices → array (p × L × num_boots)
    betaTilde_boot = simplify2array(coefs)
  } else if (boot_type == "Rao-Wu-Yue-Beaumont") {
    svy_design <- svydesign(
      ids = ~ psu + ID,
      strata = ~ strata,
      weights = ~ weight,
      data = data,
      nest = TRUE
    )
    set.seed(seed)
    rwyb_wts = make_rwyb_bootstrap_weights(
      num_replicates = num_boots,
      samp_unit_ids = svy_design$cluster,
      strata_ids = svy_design$strata,
      samp_unit_sel_probs = matrix(
        c(data$p_stage1, data$p_stage2),
        byrow = FALSE,
        ncol = 2
      ),
      samp_method_by_stage = samp_stages,
      allow_final_stage_singletons = TRUE,
      output = "weights"
    )

    coefs = lapply(1:num_boots, function(r) {
      wts_temp = rwyb_wts[, r]

      if (family$family == "gaussian") {
        # Fit all L responses at once
        coef_mat = lm_wls_multi(X_base, Y_mat, wts_temp)
      } else {
        coef_mat = glm_batch_multiY(X = X_base, y_mat = Y_mat, w = wts_temp, family = family,
        return_se = FALSE, add_intercept = FALSE)$coef
      }
      coef_mat  # (p × L)
    })
    # Convert list of matrices → array (p × L × num_boots)
    betaTilde_boot = simplify2array(coefs)
  }
  return(betaTilde_boot)

}

get_cis = function(betaTilde_boot,
                   betaHat,
                   smooth_for_ci = TRUE,
                   smooth_for_variance = TRUE,
                   L,
                   nknots_min = NULL,
                   nknots_min_cov = 35,
```

```
                  mult_fac = 1.2) {
argvals = 1:L
B = ncol(betaTilde_boot[1, , ])
nknots <- min(round(L / 2), nknots_min)
nknots_cov <- ifelse(is.null(nknots_min_cov), 35, nknots_min_cov)
nknots_fpca <- min(round(L / 2), 35)
betaHat_boot <- array(NA, dim = c(nrow(betaHat), ncol(betaHat), ncol(betaTilde_boot[1, , ])))
betaHat.var <- array(NA, dim = c(L, L, nrow(betaHat)))
# smooth


for (b in 1:B) {
  betaHat_boot[, , b] <- t(apply(betaTilde_boot[, , b], 1, function(x)
    gam(x ~ s(
      argvals, bs = "tp", k = (nknots + 1)
    ), method = "GCV.Cp")$fitted.values))
}

for (r in 1:nrow(betaHat)) {
  if (smooth_for_variance) {
    betaHat.var[, , r] <- mult_fac * var(t(betaHat_boot[r, , ]))
  } else{
    betaHat.var[, , r] <- mult_fac * var(t(betaTilde_boot[r, , ]))
  }
}

N <- 10000
qn <- rep(0, length = nrow(betaHat))
set.seed(456)
for (i in 1:length(qn)) {
  if (smooth_for_ci) {
    est_bs <- t(betaHat_boot[i, , ])
  } else{
    est_bs <- t(betaTilde_boot[i, , ])
  }
  fit_fpca <- suppressWarnings(refund::fpca.face(est_bs, knots = nknots_fpca))
  ## extract estimated eigenfunctions/eigenvalues
  phi <- fit_fpca$efunctions
  lambda <- fit_fpca$evalues
  K <- length(fit_fpca$evalues)

  ## simulate random coefficients
  theta <- matrix(stats::rnorm(N * K), nrow = N, ncol = K) # generate independent standard normals
  if (K == 1) {
    theta <- theta * sqrt(lambda) # scale to have appropriate variance
    X_new <- tcrossprod(theta, phi) # simulate new functions
  } else{
    theta <- theta %*% diag(sqrt(lambda)) # scale to have appropriate variance
    X_new <- tcrossprod(theta, phi) # simulate new functions
  }
  x_sample <- X_new + t(fit_fpca$mu %o% rep(1, N)) # add back in the mean function
  Sigma_sd <- Rfast::colVars(x_sample, std = TRUE, na.rm = FALSE) # standard deviation: apply(x_sample, 2, sd)
  x_mean <- colMeans(est_bs)
  # x_sample: N x p matrix
  # x_mean: length-p vector
  # Sigma_sd: length-p vector

  # Vectorized computation
  z <- sweep(x_sample, 2, x_mean, "-")      # center
  z <- sweep(z, 2, Sigma_sd, "/")           # standardize
  un <- apply(abs(z), 1, max)               # row-wise max of absolute values

  qn[i] <- stats::quantile(un, 0.95)
}
```

```r
  return(list(
    betaHat = betaHat,
    betaHat.var = betaHat.var,
    qn = qn
  ))

}
#
# mod_output = get_cis(res[[1]], betaHat = betaHat)
#

get_coverage_stats = function(mod_output, beta_true, name, L){
  MISE <- rowMeans((mod_output$betaHat - beta_true)^2)
  mean_pw_se = apply(mod_output$betaHat.var, 3, function(mat) mean(sqrt(diag(mat))))
  mean_joint_se <- numeric(nrow(beta_true))  # Store mean CI width

  cover_joint <- logical(nrow(beta_true))  # Using logical instead of NA-filled vector
  cover_pw <- matrix(FALSE, nrow(beta_true), L)

  # Extract the diagonal elements of each variance matrix upfront
  sqrt_diag_var <- apply(mod_output$betaHat.var, 3, function(mat) sqrt(diag(mat)))

  # Loop efficiently
  for (p in seq_along(cover_joint)) {
    true <- beta_true[p,]
    sqrt_diag_p <- sqrt_diag_var[, p]  # Extract precomputed diagonal elements

    # Compute upper and lower bounds in one step
    margin <- mod_output$qn[p] * sqrt_diag_p
    mean_joint_se[p] <- mean(margin)

    upper <- mod_output$betaHat[p,] + margin
    lower <- mod_output$betaHat[p,] - margin

    margin_pw <- 1.96 * sqrt_diag_p
    upper_pw <- mod_output$betaHat[p,] + margin_pw
    lower_pw <- mod_output$betaHat[p,] - margin_pw

    # Compute joint and pointwise coverage efficiently
    covered <- (lower < true) & (upper > true)
    covered_pw <- (lower_pw < true) & (upper_pw > true)

    cover_joint[p] <- all(covered)  # Joint coverage check
    cover_pw[p, ] <- covered_pw     # Assign logical vector directly
  }

  tibble(
    MISE = MISE %>% unname(),
    mean_joint_se = mean_joint_se,
    mean_pw_se = mean_pw_se,
    cover_joint = cover_joint,
    cover_pw = rowSums(cover_pw),
    var = rownames(beta_true),
    boot_type = name)
}


get_coverage_stats_fui = function(mod_output, beta_true, L){
  MISE <- rowMeans((mod_output$betaHat - beta_true)^2)
  mean_pw_se = apply(mod_output$betaHat.var, 3, function(mat) mean(sqrt(diag(mat))))
  mean_joint_se <- numeric(nrow(beta_true))  # Store mean CI width

  cover_joint <- logical(nrow(beta_true))  # Using logical instead of NA-filled vector
  cover_pw <- matrix(FALSE, nrow(beta_true), L)
```

```r
  # Extract the diagonal elements of each variance matrix upfront
  sqrt_diag_var <- apply(mod_output$betaHat.var, 3, function(mat) sqrt(diag(mat)))

  # Loop efficiently
  for (p in seq_along(cover_joint)) {
    true <- beta_true[p,]
    sqrt_diag_p <- sqrt_diag_var[, p]  # Extract precomputed diagonal elements

    # Compute upper and lower bounds in one step
    margin <- mod_output$qn[p] * sqrt_diag_p
    mean_joint_se[p] <- mean(margin)

    upper <- mod_output$betaHat[p,] + margin
    lower <- mod_output$betaHat[p,] - margin

    margin_pw <- 1.96 * sqrt_diag_p
    upper_pw <- mod_output$betaHat[p,] + margin_pw
    lower_pw <- mod_output$betaHat[p,] - margin_pw

    # Compute joint and pointwise coverage efficiently
    covered <- (lower < true) & (upper > true)
    covered_pw <- (lower_pw < true) & (upper_pw > true)

    cover_joint[p] <- all(covered)  # Joint coverage check
    cover_pw[p, ] <- covered_pw     # Assign logical vector directly
  }
  cover_pw_int = which(cover_pw[1, ])
  cover_pw_x = which(cover_pw[2, ])
  result = tibble(
    MISE = MISE %>% unname(),
    mean_joint_se = mean_joint_se,
    mean_pw_se = mean_pw_se,
    cover_joint = cover_joint,
    cover_pw = rowSums(cover_pw) / L,
    var = rownames(beta_true)) %>%
    mutate(vector_col = map(var, ~ ifelse(.x  == "Intercept", list(cover_pw_int), list(cover_pw_x))))
  return(result)

}


get_coverage_stats_famm = function(res, beta_true, L = 50){
  coef_pffr = coef(res, n1 = L)
  betaHat_pffr <- betaHat_pffr.se <- matrix(NA, nrow = 2, ncol = L)
  betaHat_pffr[1,] = as.vector(coef_pffr$smterms$`Intercept(yindex)`$value) + unname(res$coef[1])
  betaHat_pffr[2,] = as.vector(coef_pffr$smterms$`X(yindex)`$value)
  betaHat_pffr.se[1,] = as.vector(coef_pffr$smterms$`Intercept(yindex)`$se)
  betaHat_pffr.se[2,] = as.vector(coef_pffr$smterms$`X(yindex)`$se)
  MISE = rowMeans((betaHat_pffr - beta_true)^2)
  mean_pw_se = apply(betaHat_pffr.se, 1, mean)

  cover_pw = matrix(FALSE, nrow(beta_true), L)
  for(p in seq_along(MISE)){
    cover_upper = which((betaHat_pffr[p,]+(1.96*betaHat_pffr.se[p,])) > beta_true[p,])
    cover_lower = which((betaHat_pffr[p,]-(1.96*betaHat_pffr.se[p,])) < beta_true[p,])
    cover_pw[p, intersect(cover_lower, cover_upper)] = TRUE
  }

  cover_pw_int = which(cover_pw[1, ])
  cover_pw_x = which(cover_pw[2, ])


  tibble(
    MISE = MISE %>% unname(),
    mean_pw_se = mean_pw_se,
```

```
    cover_pw = rowSums(cover_pw) / L,
    var = rownames(beta_true)) %>%
    mutate(vector_col = map(var, ~ ifelse(.x  == "Intercept", list(cover_pw_int), list(cover_pw_x))))
}
```

## 3. CODE FOR RUNNING SIMULATION

```
library(future)
library(furrr)
library(tidyverse)
library(here)
library(devtools)
library(fastFMM)
library(haven)
library(survey)
library(progress)
library(lme4)
library(paletteer)
library(mgcv)
library(ggplot2)
library(gridExtra)
library(tidyfun)
library(mvtnorm)
library(refund)
library(svrep)
source(here::here("R_cp", "01_sim_functions.R"))
source(here::here("R_cp", "00_data_gen_function_ff.R"))
source(here::here("R", "utils.R"))
source(here::here("R_cp", "create_survey_settings.R"))


force = FALSE
force_iter = FALSE
nsim = 200
B = 500
# ncores = parallelly::availableCores()
ncores = future::availableCores()

fit_types = c('weighted', 'unweighted')
boot_types = c('Rao-Wu-Yue-Beaumont', 'BRR', 'weighted', 'unweighted')
options(survey.lonely.psu = "adjust")


ifold = get_fold()

outfile = here::here("results", "simulations", "survey_sim", paste0("fold_", sprintf("%03d", ifold), ".rds"))

if(!file.exists(outfile) || force) { # if the file doesn't exist or we want to force re-do it
  if (!dir.exists(dirname(outfile))) dir.create(dirname(outfile), recursive = TRUE)
  partial_dir = here::here("results", "simulations", "survey_sim",
  paste0("fold_", sprintf("%03d", ifold), "_partials"))
  if (!dir.exists(partial_dir)) dir.create(partial_dir)

  temp = settings_new[ifold,]


  lst = generate_superpopulation(
    scenario = temp$scenario,
    family = temp$family,
    I = 10e6,
    L = temp$len,
    snr_b = temp$snr_b,
    snr_eps = temp$snr_eps,
    strata_sigma = temp$strata_sigma,
    strata_scale = temp$strata_scale,
    seed = 111
```

```r
)


plan(multisession, workers = ncores)

# check for completed iters
completed_iters = list.files(partial_dir, pattern = "^iter_\\d+\\.rds$") %>%
  str_extract("\\d+") %>%
  as.integer()

for (iter in 1:nsim) {
  if (iter %in% completed_iters && !force_iter) {
    message("Skipping completed iteration: ", iter)
    next
  }

  set.seed(iter)
  x = try({
    data = sample_from_population_wor(
      X_des = lst$X_des,
      Y_obs = lst$Y_obs,
      L = temp$len,
      I_n = temp$In,
      num_strata = 30,
      stratum_assignments = lst$stratum_assignments,
      psu_assignments = lst$psu_assignments,
      dirichlet_probs = lst$dirichlet_probs,
      seed = iter,
      inf_level = temp$inf_level,
      compression = 2,
      family = temp$family
    )
    print(summary(data$weight))

    beta_true = lst$beta_true
    betaTilde = map(
      .x = fit_types,
      .f = get_betatilde,
      data = data,
      family = temp$family
    )

    betaHat = map(.x = betaTilde, get_betahat, L = temp$len)


    res = future_map(
      .x = boot_types,
      .f = run_boots_xfast,
      betaHat = betaHat[[1]], # don't actually use betahat in calculation so we can just use the weighted one
      data = data,
      family = temp$family,
      num_boots = B,
      seed = 2025,
      L = temp$len,
      samp_stages = c("PPSWOR", "Poisson"),
      .options = furrr_options(seed = TRUE)
    )

    fit_list = list(betaHat[[1]], betaHat[[1]], betaHat[[1]], betaHat[[2]])

    cis = future_map2(
      .x = res,
      .y = fit_list,
      .f = get_cis,
      L = temp$len,
```

```
      smooth_for_ci = TRUE,
      .options = furrr_options(seed = TRUE)
    )

    stats = future_map2(
      .x = cis,
      .y = boot_types,
      .f = get_coverage_stats,
      beta_true = beta_true,
      L = temp$len
    ) %>%
      list_rbind() %>%
      mutate(n = nrow(data), n_boot = B)


    write_rds(stats, file = file.path(partial_dir, sprintf("iter_%03d.rds", iter)))

  })
  rm(x)
  print(iter)
}

plan(sequential)

partial_files = list.files(partial_dir, pattern = "^iter_\\d+\\.rds$", full.names = TRUE)

sim_res = map(partial_files, \(x) read_rds(x) %>%
mutate(id = sub(".*iter_(.+)\\.rds.*", "\\1", basename(x)))) %>%
  keep(., is.data.frame) %>%
  list_rbind()

write_rds(sim_res, file = outfile)


unlink(partial_dir, recursive = TRUE)
}
```
