# Supplementary material for: Function on Scalar Regression with Complex Survey Designs
Source: arXiv:2511.05487 source file (2026-10-06)
Supplement: Supplementary file 3 [file Web_Appendix_C.pdf]

# Web Appendix C: Analytical Simulation Vignette

## Overview

The goal of the simulation is to (1) generate a superpopulation of individuals and then (2) sample from the superpopulation.

Let's break down each step.

1. Generate a superpopulation of individuals

- Each individual belongs to a stratum and PSU within the stratum
  - These strata/PSUs can be thought of as geographical areas and towns within those areas
- Each individual has covariates and a functional outcome
- Functional outcomes may be correlated within strata and PSUs

2. Sample from the superpopulation

- Sample two PSUs from each stratum
- Sample individuals within the selected PSUs
- The sampling may be informative, meaning that the probability of selection may depend on the outcome

Once we have obtained the sample, we fit the model to the data in the sample. We compare the estimate for the model to the true data generating mechanism in the superpopulation.

We'll walk through each step below, using a smaller superpopulation size to make the computations faster.

### Generate superpopulation

In the manuscript, we create a superpopulation of size $I = 10^7$. For illustration purposes in this vignette, we set $I = 10^6$.

#### Assignment to strata and PSU

We'll start by generating the stratum and PSU assignments for the individuals in the superpopulation. We assign individuals to strata and PSUs using Dirichlet probabilities with concentration parameter 4 and 10, respectively. The concentration parameter controls the uniformity of the probabilities. On average, with 30 strata and $10^7$ individuals, the smallest probability of belonging to a stratum is 0.009, and the largest probability is 0.076 We choose $H = 30$ strata and between 75 and 125 PSUs per stratum.

```
I = 10e5 # superpopulation size
num_strata = 30 # number of strata
min_psu = 75
max_psu = 125
seed = 2213
set.seed(seed)
# generate dirichlet probabilities for stratum assignments
# using concentration param 4
dirichlet_probs = gtools::rdirichlet(1, rep(4, num_strata))
set.seed(seed)
# generate stratum assignments
stratum_assignments = sample(1:num_strata, I, replace = TRUE,
                             prob = dirichlet_probs)
psu_assignments  = rep(NA, I)

# loop thru strat and assign individuals to PSUs
# between 75 and 125 psus per stratum
for (s in 1:num_strata) {
  set.seed(seed + s)
  num_in_strata = sum(stratum_assignments == s)
  num_psu = round(runif(1, min_psu, max_psu), 0)
  set.seed(seed + s)
  dps = gtools::rdirichlet(1, rep(10, num_psu))
  set.seed(seed + s)
  psu_in_stratum = sample(1:num_psu,
                          num_in_strata,
                          replace = TRUE,
                          prob = dps)
```

```
  psu_assignments[stratum_assignments == s]  = paste0(s, "_", psu_in_stratum)
}
```

We can visualize the strata and PSUs:

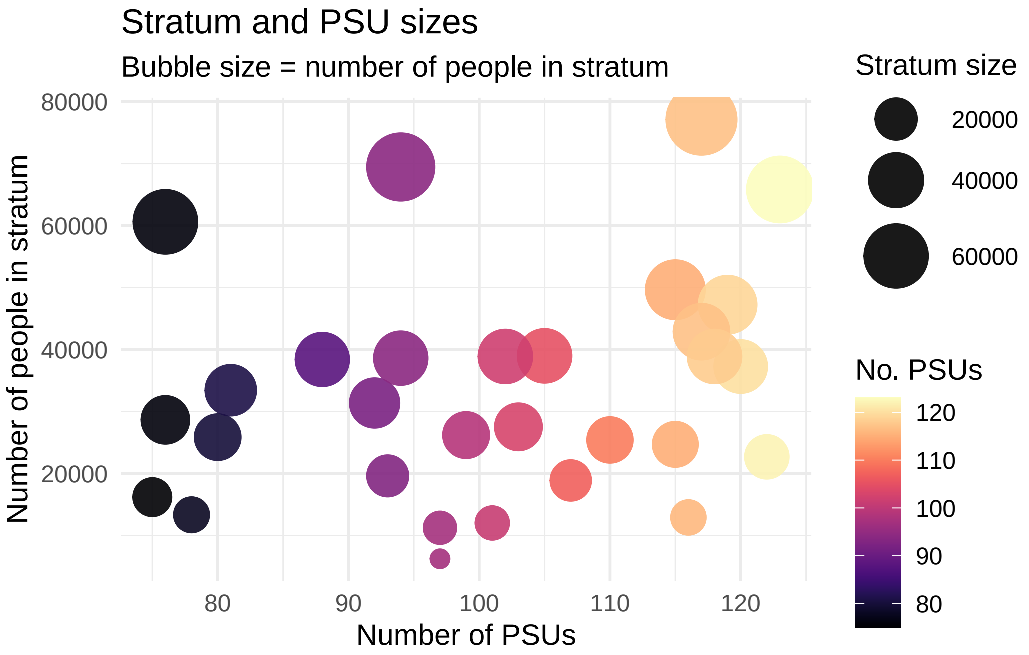


#### Generate covariates and baseline linear predictors

We assign each individual a covariate sampled from a Normal distribution: $X_i \sim \mathcal{N}(0, 2)$. We create a baseline linear predictor for each individual that is a function of the covariate and global intercept and slope functions:

$$\eta_i(s) = g\{\mu_i(s)\} = \beta_0(s) + X_i\beta_1(s)$$

Where $\beta_0(s)$ is a global intercept function and $\beta_1(s)$ is a slope function. In particular:

$$\beta_0(s) = 0.53 + 0.06\sin(3\pi s) - 0.03\cos(6.5\pi s)$$

$$\beta_1(s) = \frac{1}{20}\phi\Big(\frac{s - 0.6}{0.0225}\Big)$$

Where $\phi(\cdot)$ is the standard normal pdf.

```r
# generate X
set.seed(seed)
X_des = cbind(1, rnorm(I, 0, 2))

# generate global intercept and slope functions
L = 50 # length of functional domain
grid  = seq(0, 1, length = L)
beta_fixed  = matrix(NA, 2, L)

beta_fixed[1, ]  = -0.15 - 0.1 * sin(2 * pi * grid) - 0.1 * cos(2 * pi * grid)
beta_fixed[2, ]  = dnorm(grid, 0.6, 0.15) / 20

rownames(beta_fixed)  = c("Intercept", "x")
```

We can plot the global intercept and slope functions:

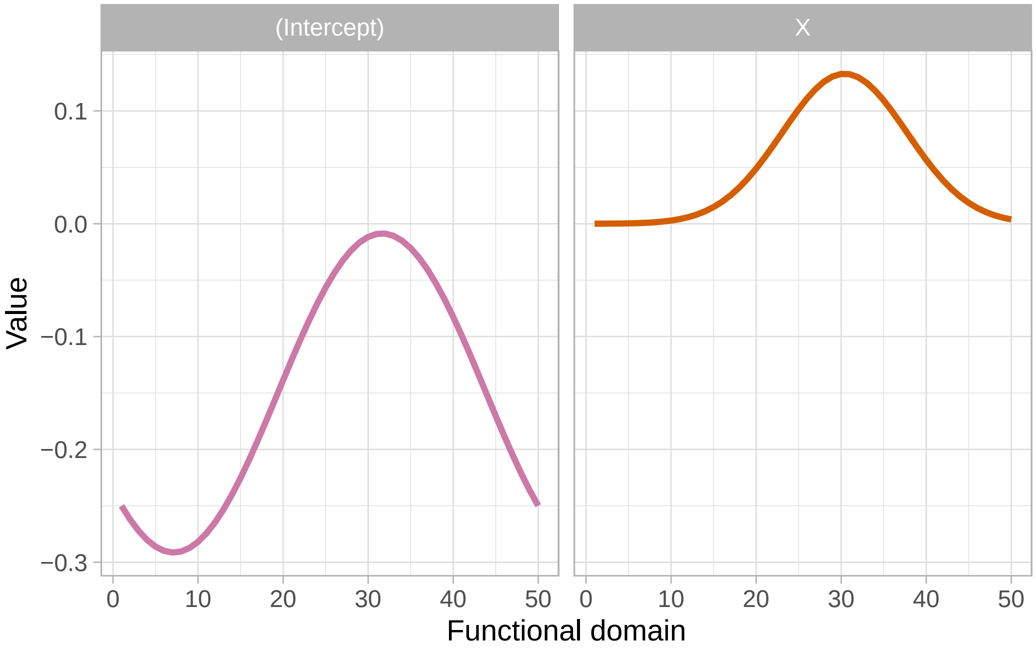


#### Add stratum/PSU specific noise

Next, we (optionally) add strata and PSU specific noise. We have two ways we can do this: (1) scale or shrink the coefficient function, (2) add strata/PSU-specific functional random effects. We'll walk through the implementation of both.

#### Stratum-specific slope scaling

Recall that $\beta_1(s)$ is the global slope function. We can create a stratum-specific slope function by scaling the global slope function by a stratum-specific random variable:

$$\beta_{1(h)}(s) = \gamma_h \cdot \beta_1(s)$$

Where $\gamma_h \sim N(1, 0.125^2)$

```
# add stratum-specific slope modifications
set.seed(seed)
strata_scale = 0.125
stratum_scaling  = rnorm(num_strata, mean = 1, sd = strata_scale)

beta1_by_stratum  = matrix(rep(stratum_scaling, each = L), nrow = num_strata,
                           byrow = TRUE) *
  matrix(rep(beta_fixed[2, ], times = num_strata),
         nrow = num_strata,
         byrow = TRUE) # num_strata x L matrix

# assign to individuals
beta1_by_indiv  = beta1_by_stratum[stratum_assignments, ]
```

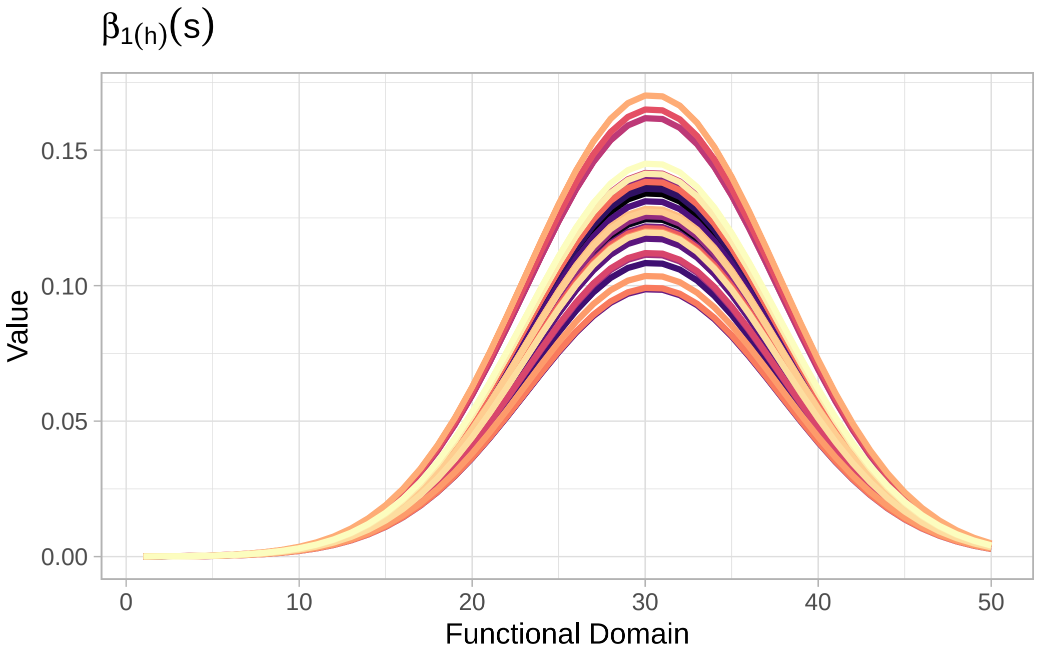

### Adding stratum and PSU-specific noise

To create within-stratum correlation, we simulate functional random effects at the strata level. Let $\{\phi_k(s)\}_{k=1}^K$ be a B-spline basis of dimension $K = 5$ over $[0,1]$, $b_h(s) = \sum_{k=1}^K \xi_{hk}\phi_k(s)$ be the stratum-level random effect and $b_{c(h)}(s) = \sum_{k=1}^K \zeta_{gk}\phi_k(s)$ be the PSU-level random effect for PSU $c$ nested within stratum $h$. The spline coefficients are simulated from $\xi_{hk} \sim N(0, \sigma_h^2)$ and $\zeta_{gk} \sim N(0, \sigma_h^2/2)$, where $\sigma_h = 0.05$.

We implement as follows:

```
strata_sigma = 0.05 # stratum-specific noise
psu_factor = 0.5 # importance of PSU effect relative to strata effect
psu_sigma = sqrt(strata_sigma ^ 2 * psu_factor) # psu-specific noise

# create strata-specific random effects
nbasis  = 5
basis  = fda::create.bspline.basis(c(0, 1), nbasis)
Phi  = fda::eval.basis(grid, basis)
```

We can plot the basis functions:

```
plot(basis)
```

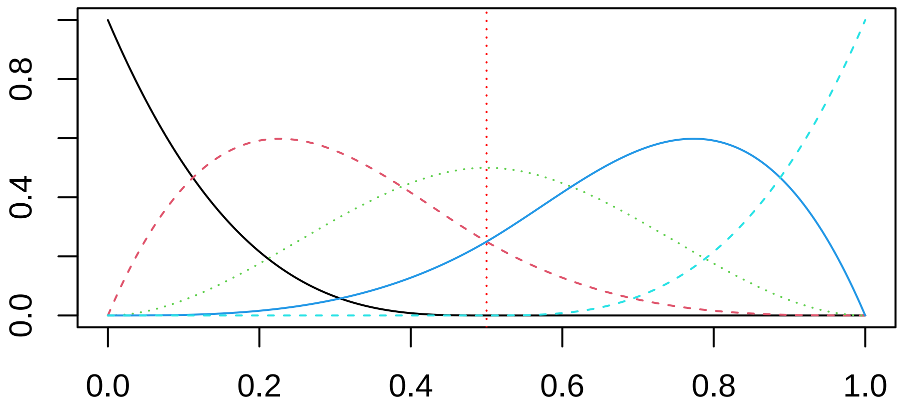


```
set.seed(seed)
strata_scores  = matrix(rnorm(num_strata * nbasis, 0, strata_sigma),
                        num_strata,
                        nbasis) # num_strata x nbasis matrix

strata_random_effects  = strata_scores %*% t(Phi) # num_strata x nbasis matrix
```

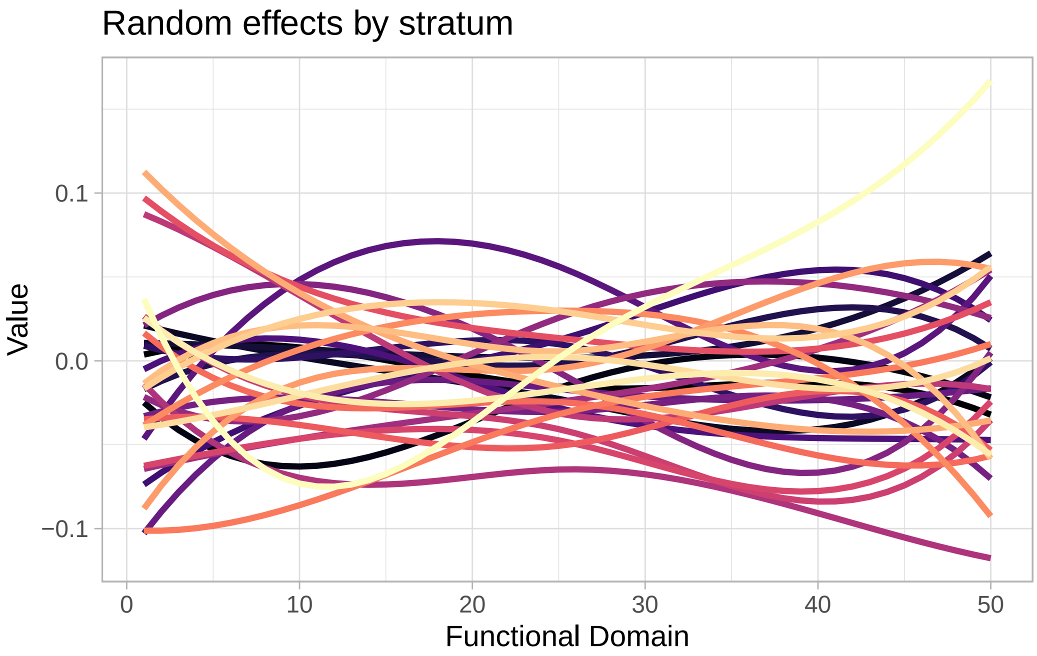


Now the PSU-level random effects:

```
total_psu = length(unique(psu_assignments))

set.seed(seed)
psu_scores  = matrix(rnorm(total_psu * nbasis, 0, psu_sigma),
                     total_psu, nbasis)
psu_random_effects  = psu_scores %*% t(Phi)
```

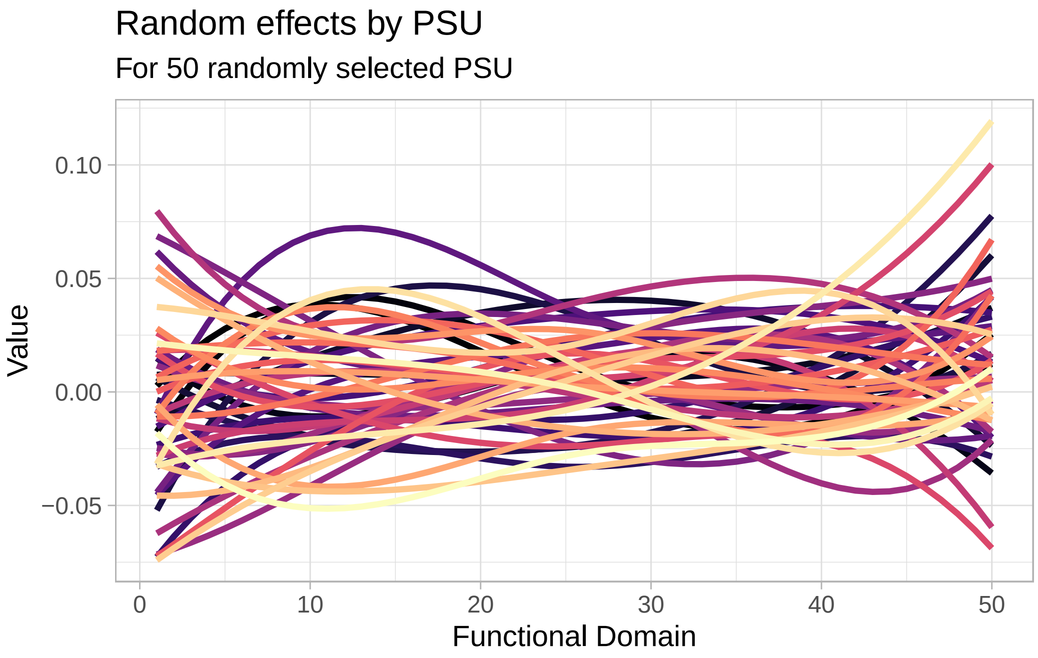


**Combine to get linear predictors**

We adjust the random effects to achieve the desired relative importance of the random effects (ratio of standard deviation of random effects to standard deviation of fixed effects), `snr_b`.

The individual-level linear predictor is:

$$\eta_i(s) = \beta_0(s) + X_i\beta_{1(h)}(s) + b_{h(i)}(s) + b_{c(h,i)}(s)$$

```
snr_b = 1

# adjust random effect based on relative importance of random effects
fixef_signal  = matrix(rep(beta_fixed[1, ], I), nrow = I, byrow = TRUE) +
  X_des[, 2] * matrix(rep(beta_fixed[2, ], I), nrow = I, byrow = TRUE)

# include stratum-specific slope variation in the random effects
slope_re  = (stratum_scaling[stratum_assignments] - 1) *
  matrix(rep(beta_fixed[2, ], I), nrow = I, byrow = TRUE)

strata_effects_indiv  = strata_random_effects[stratum_assignments, ]
psu_effects_indiv  = psu_random_effects[as.numeric(factor(psu_assignments)), ]
random_effects  = strata_effects_indiv + psu_effects_indiv
```

```
ranef   = slope_re + random_effects
ranef   = sd(fixef_signal) / sd(ranef) / snr_b * ranef
rm(random_effects)
lin_pred = fixef_signal + ranef
```

We can plot the fixed effects, random effects, and linear predictors:

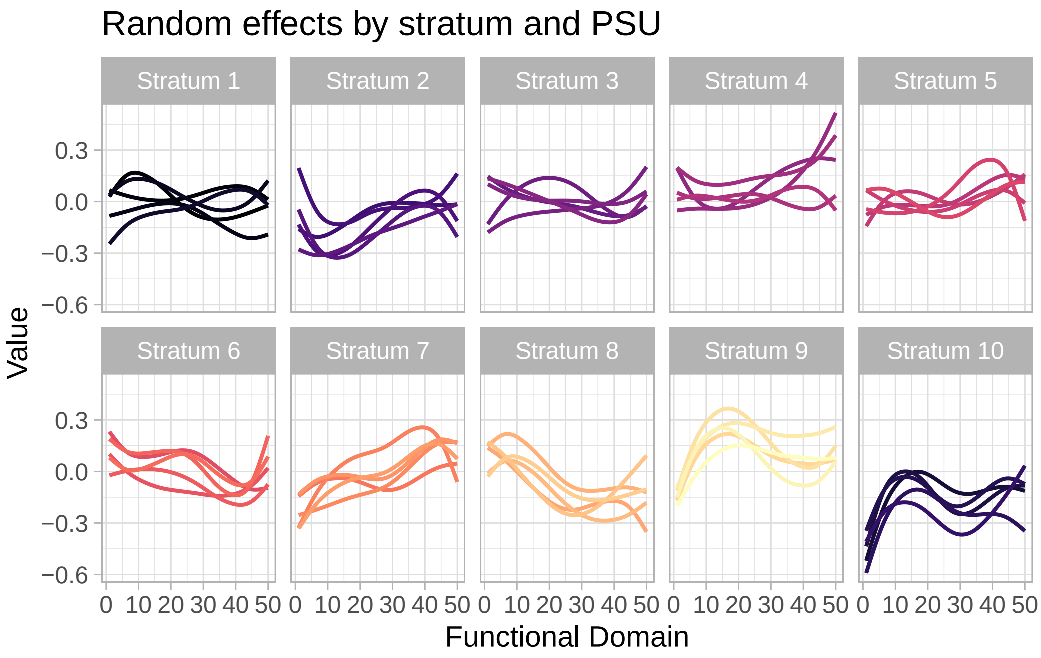

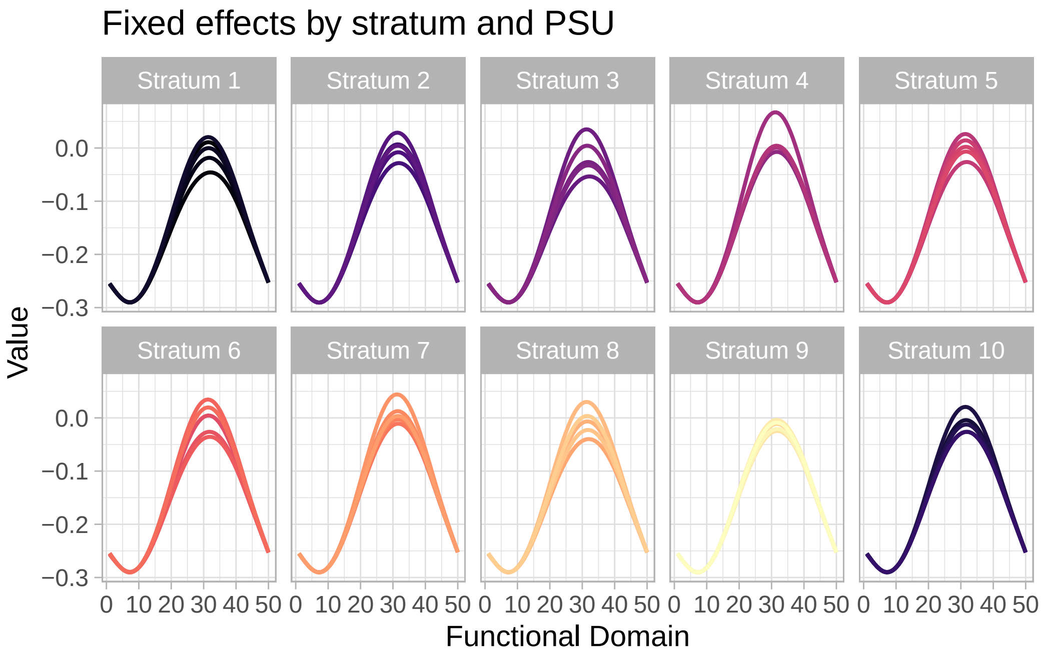


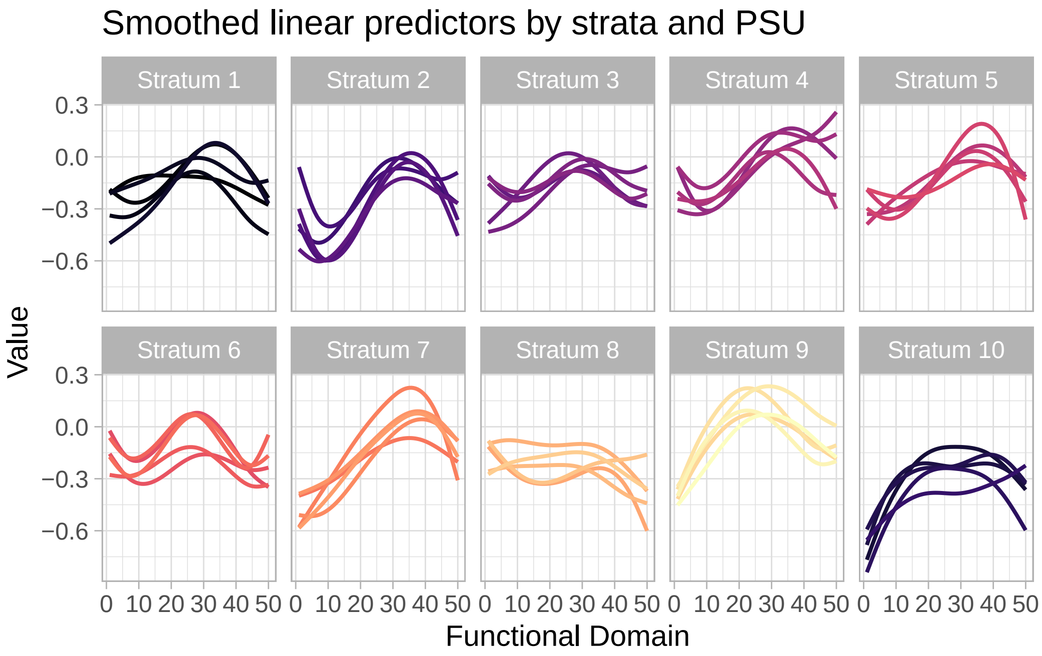


### Generate outcomes from linear predictors

Now that we have linear predictors with stratum and PSU specific noise, we can generate the outcomes for each individual.

For Gaussian data, we obtain outcomes by sampling from a Normal distribution with mean $\eta_i(s)$ and standard deviation $\sigma^2$, where $\sigma^2$ is varied to account for different levels of the signal to noise ratio. For binary data, outcomes are sampled independently from a Bernoulli distribution with probability $p_i(s) = \frac{e^{\eta_i(s)}}{1+e^{\eta_i(s)}}$. For count data, outcomes are sampled independently from a Poisson distribution with mean $e^{\eta_i(s)}$.

```
family = "gaussian"
snr_eps = 1
if (family == "gaussian") {
  sd_lp = sd(lin_pred)
  sigma = sd_lp / snr_eps
  set.seed(seed)
  Y_obs = matrix(
    rnorm(
      n = I * L,
      mean = as.vector(t(lin_pred)),
      sd = sigma
    ),
    # need to use t to put in correct order
    nrow = I,
    ncol = L,
    byrow = TRUE
  )
} else if (family == "binomial") {
  p_true = plogis(as.vector(t(lin_pred)))
  set.seed(seed)
  Y_obs  = matrix(
    rbinom(n = I * L, size = 1, prob = p_true),
    nrow = I,
    ncol = L,
    byrow = TRUE
  )
} else if (family == "poisson") {
  lam_true = exp(as.vector(t(lin_pred)))
  set.seed(seed)
  Y_obs  = matrix(
    rpois(n = I * L, lambda = lin_pred_vec),
    nrow = I,
    ncol = L,
    byrow = TRUE
  )
}
```

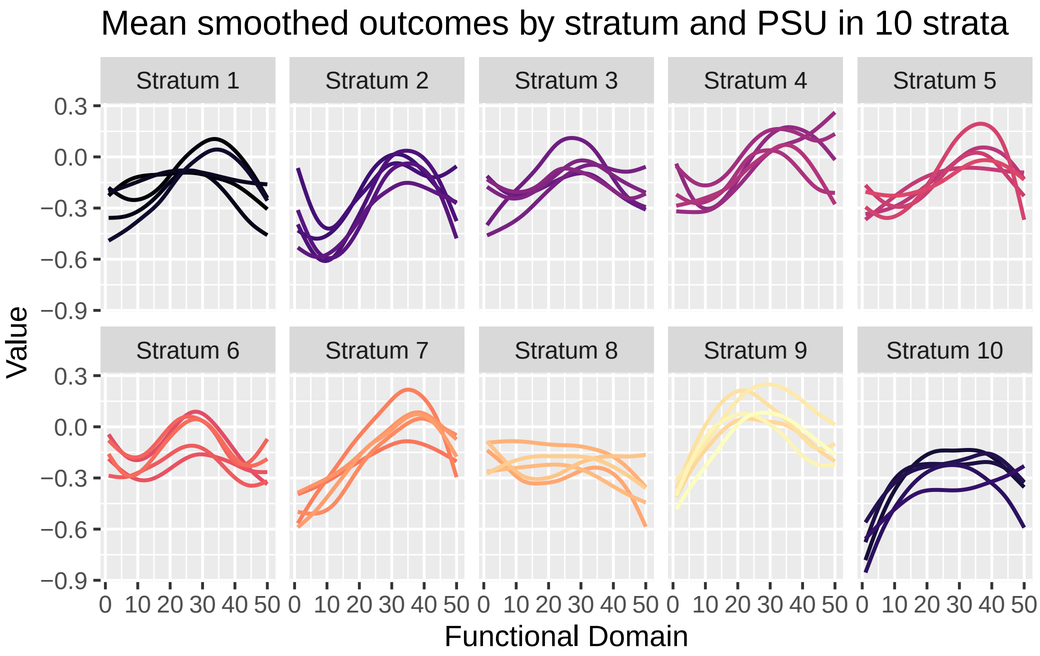


### Sample from superpopulation

We sample from the super population to simulate a two-stage sampling design with probability proportional to size without replacement (PPSWOR) at the first stage (sampling PSUs from strata) and Poisson sampling at the second stage (sampling individuals from selected PSUs).

#### Sample PSU from strata

We sample two psu from each stratum, without replacement, where the probability of selection is proportional to the number of individuals in the PSU. For now, we'll focus on only one stratum.

```
# function to calculate inclusion probability sampling without replacement
get_p_i = function(i, probs) probs[i] * (1 + sum((probs[-i]) / (1-probs[-i])))

num_selected_psu = 2 # we want to select 2 PSUs
X1 = X_des[, 2] # covariate to use for informative sampling

strata = 1 # just focus on first stratum
inds_in_stratum  = which(stratum_assignments == strata) # individuals in stratum

# Get PSU sizes in this stratum
```

```r
psu_sizes = table(psu_assignments[inds_in_stratum])
psu_ids = names(psu_sizes)

# Sample PSUs WITH replacement using PPS
set.seed(strata + seed)
selected_psus = sample(psu_ids,
                       size = num_selected_psu,
                       replace = FALSE,
                       prob = psu_sizes)

psu_probs  = psu_sizes / sum(psu_sizes)  # the pps probabilities
# the selection probabilities
psu_prob_selected = map_dbl(.x = match(selected_psus, psu_ids),
                            .f = get_p_i,
                            psu_probs)

names(psu_prob_selected) = selected_psus
psu_prob_selected # which PSU did we select
```

```
      1_74       1_26
0.02662360 0.02776188
```

#### Sample individuals from PSU

To sample individuals from each PSU, we use Poisson sampling, where each individual has a separate inclusion probability. Under informative sampling, we generate the inclusion probabilities as a function of the mean of each individual's outcome. Under non-informative sampling, each individual is assigned the same inclusion probability. We adjust the inclusion probabilities such that we select the desired number of individuals from each PSU.

Let $\overline{Y}_i = \sum_{l=1}^{L} Y_i(s_l)$ denote the mean of the functional outcome for individual $i$ and let $k$ be a scalar that controls the degree of informativeness in the sampling scheme, with larger values of $k$ corresponding to stronger informativeness. We generate an inclusion score $s_i$ as follows:

- Gaussian data: $s_i = k\overline{Y}_i$
- Bernoulli data: $s_i = k \log\left(\frac{\overline{Y}_i}{1-\overline{Y}_i}\right)$
- Poisson data: $s_i = k \log(\overline{Y}_i)$

Next, we truncate the scores $s_i$ to be between $-2$ and 2: $s'_i = \max(\min(s_i, 2), -2)$, then map the scores to inclusion probabilities using the logistic function: $\pi_i = \frac{1}{1+e^{-s'_i}}$.

The $\pi_i$ are adjusted to ensure the desired amount of individuals per stratum/PSU combination. Let $I_n$ denote the desired number of individuals selected per PSU. Then the adjusted inclusion probabilities are: $\pi_i^* = \min\left(1, \frac{I_n \pi_i}{\sum_k^{I_{h,c}} \pi_k}\right)$.

We'll walk through the implementation, focusing on the first PSU we selected, PSU 47 in stratum 1.

```r
psu = selected_psus[1]
compression = 2
I_n = 50 # number of individuals targeted to select from each PSU
inf_level = 10 # strength of "informativeness"
# individuals in the PSU/stratum
inds_in_psu  = which(psu_assignments == psu & stratum_assignments == strata)


if (inf_level == 0) {
  # Uniform sampling
  n = length(inds_in_psu)
  inclusion_probs = rep(1 / n, n)
} else {
  # Compute mean outcome in PSU
  y_mean = rowMeans(Y_obs[inds_in_psu, ])

  # Compute inclusion score depending on family
  incl_score = switch(
    family,
    "gaussian" = y_mean * inf_level,
    "poisson"  = log(y_mean) * inf_level,
    "binomial" = qlogis(pmin(pmax(y_mean, 1e-6), 1 - 1e-6)) * inf_level,
    stop("Unknown family")
  )

  # Apply compression and map to probabilities
  score_compressed = pmax(pmin(incl_score, compression), -compression)
  inclusion_probs = plogis(score_compressed)
}
# adjust by I_n
inclusion_probs_adj  = inclusion_probs / sum(inclusion_probs) * I_n
# truncate at 1
inclusion_probs_adj[inclusion_probs_adj > 1]  = 1

set.seed(strata + seed + which(selected_psus == psu)) # ensure reproducibility
# poisson sampling
```

```
sampled_units  = inds_in_psu[rbinom(length(inds_in_psu), 1,
                                    inclusion_probs_adj) == 1]
```

We can examine the difference between the adjusted an unadjusted probabilities, to confirm that the adjustment shifts the probabilities lower so that we select, on average, 50 individuals.

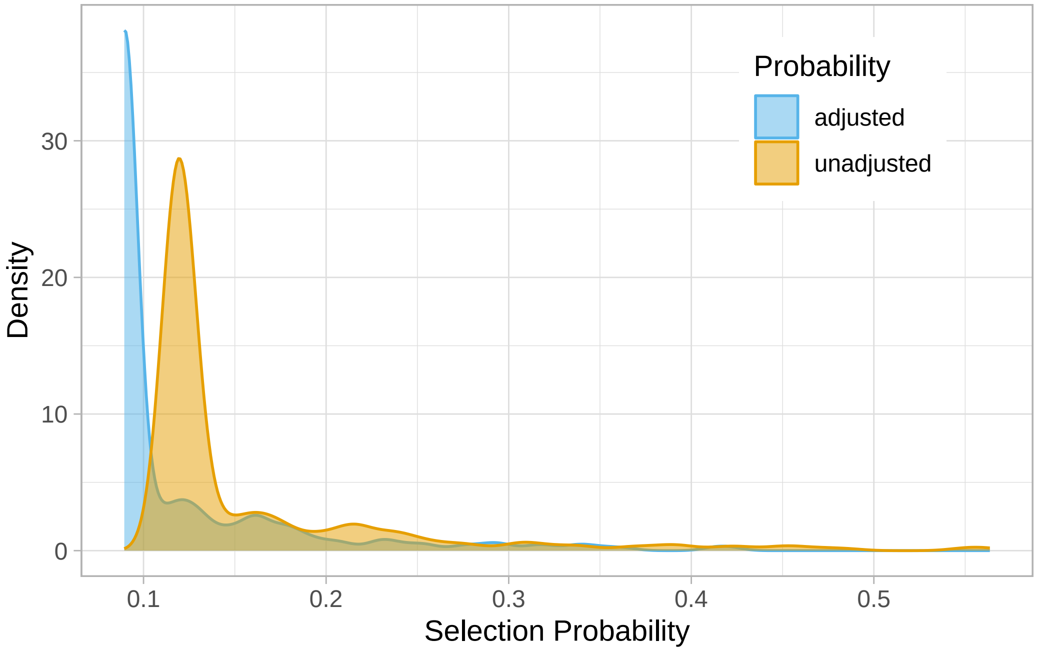


#### Repeat across strata and PSU to get full sample

We repeat in each strata to get the entire sample, storing the selection probability at each stage. The final selection probability is the product of the stage 1 (sampling PSU) and stage 2 (sampling individuals) selection probabilities. The final survey weight is the reciprocal of the selection probability.

```
p_strata_design  = dirichlet_probs
final_sample  = c() # to store final sample ids
p1  = rep(NA, I) # stage 1 selection probability
p2  = rep(NA, I) # stage 2 selection probability
p_overall  = rep(NA, I) # overall selection probability
psus  = c() # to store PSUs

# within each strata, select PSU with replacement using PPS
```

```
for (strata in 1:num_strata) {
  # strata = 1
  # individuals in the strata
  inds_in_stratum  = which(stratum_assignments == strata)

  # Get PSU sizes in this stratum
  psu_sizes = table(psu_assignments[inds_in_stratum])
  psu_ids = names(psu_sizes)

  # Sample PSUs WITH replacement using PPS
  set.seed(strata + seed)
  selected_psus = sample(psu_ids,
                        size = num_selected_psu,
                        replace = FALSE,
                        prob = psu_sizes)

  psu_probs  = psu_sizes / sum(psu_sizes)  # PPS
  # probability of selection is 1 - (p(not selected both times))
  # psu_prob_selected  = 1 - (1 - psu_probs) ^ num_selected_psu
  # names(psu_prob_selected)  = psu_ids

  psu_prob_selected = map_dbl(.x = match(selected_psus, psu_ids),
                              .f = get_p_i,
                              psu_probs)

  names(psu_prob_selected)  = selected_psus
  # within each selected PSU select individuals based on X1
  for (psu in selected_psus) {
    inds_in_psu  = which(psu_assignments == psu &
                         stratum_assignments == strata)
    if (inf_level == 0) {
      # Uniform sampling
      n = length(inds_in_psu)
      inclusion_probs = rep(1 / n, n)
    } else {
      # Compute mean outcome in PSU
      y_mean = rowMeans(Y_obs[inds_in_psu, ])

      # Compute inclusion score depending on family
      incl_score = switch(
        family,
        "gaussian" = y_mean * inf_level,
```

```r
        "poisson"  = log(y_mean) * inf_level,
        "binomial" = qlogis(pmin(pmax(y_mean, 1e-6), 1 - 1e-6)) * inf_level,
        stop("Unknown family")
      )

      # Apply compression and map to probabilities
      score_compressed = pmax(pmin(incl_score, compression), -compression)
      inclusion_probs = plogis(score_compressed)
    }
    inclusion_probs_adj  = inclusion_probs / sum(inclusion_probs) * I_n
    inclusion_probs_adj[inclusion_probs_adj > 1]  = 1

    set.seed(strata + seed + which(selected_psus == psu)) # ensure reproducibility
    sampled_units  = inds_in_psu[rbinom(length(inds_in_psu), 1,
                                    inclusion_probs_adj) == 1]

    final_sample  = c(final_sample, sampled_units)
    psus  = c(psus, rep(psu, length(sampled_units)))
    p_psu  = psu_prob_selected[which(names(psu_prob_selected) == psu)]

    p1[inds_in_psu]  = p_psu
    p2[inds_in_psu]  = inclusion_probs_adj
    p_overall[inds_in_psu]  = p_psu * inclusion_probs_adj
  }
}


survey_weights  = 1 / p_overall


dat.sim  = data.frame(
  ID = final_sample,
  X = X1[final_sample],
  strata = stratum_assignments[final_sample],
  psu = sub(".*\\_", "", psus),
  weight = survey_weights[final_sample],
  p_stage1 = p1[final_sample],
  p_stage2 = p2[final_sample]
)
Y_sample = Y_obs[final_sample, ]
```

Let $\pi_i^*$ denote the normalized, scaled, and truncated probability of selecting individual $i$ within

PSU $c(h)$, and $\pi_{c(h)}$ denote the probability of selecting PSU $c$ from stratum $h$. Each selected individual is assigned a survey weight $w_{hci} = 1/(\pi_i^* \pi_{c(h)})$. These are the weights we will use in subsequent analysis.

We can examine the distribution of survey weights and the mean outcome by tertile of survey weight. Since we employed informative sampling, we expect to see differences in the outcome by survey weight.

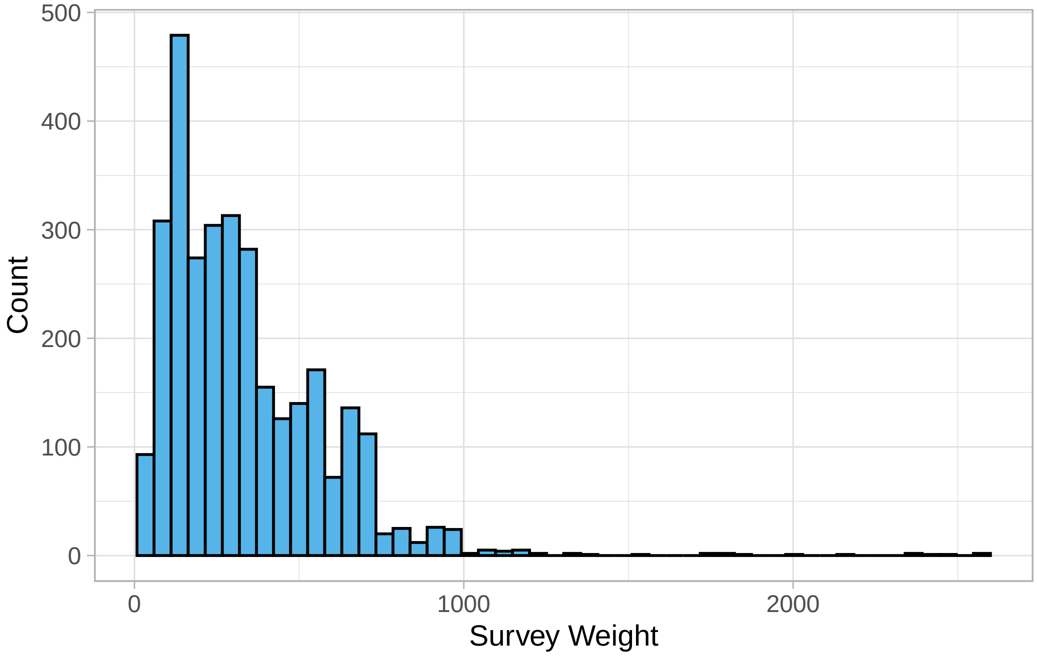

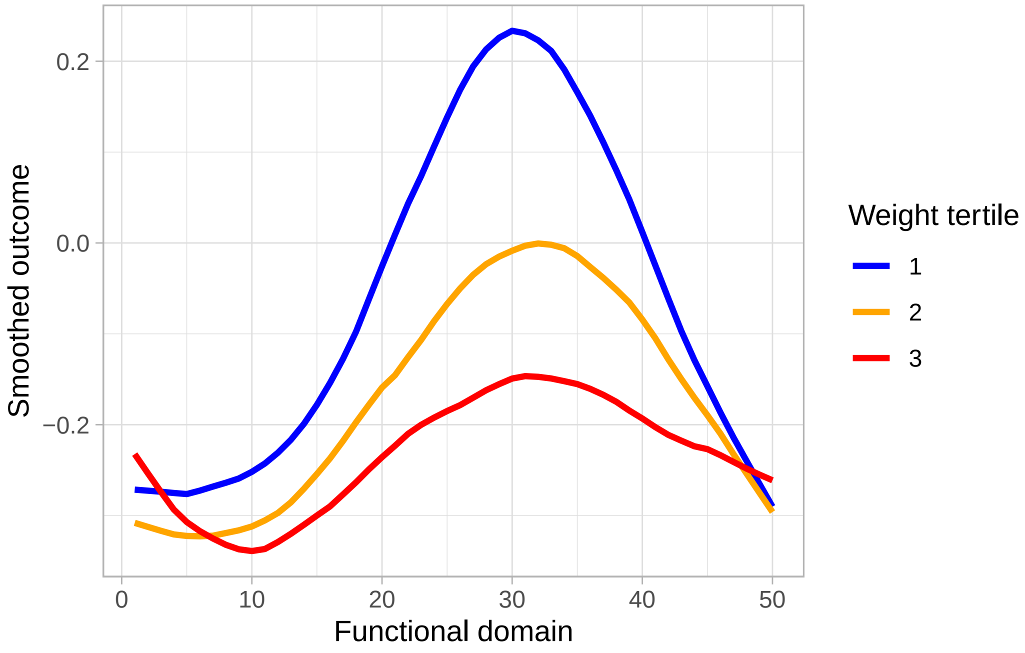

Smoothed outcome
0.2
0.0
−0.2
0
10
20
30
40
50
Functional domain
Weight tertile
1
2
3
