# Supplementary material for: Function on Scalar Regression with Complex Survey Designs
Source: arXiv:2511.05487 source file (2026-10-06)
Supplement: Supplementary file 4 [file Web_Appendix_D.pdf]

# Web Appendix D: Supplemental Tables and Figures

## 1. MISE

### A. Gaussian data

#### *A.1. Functional intercept*

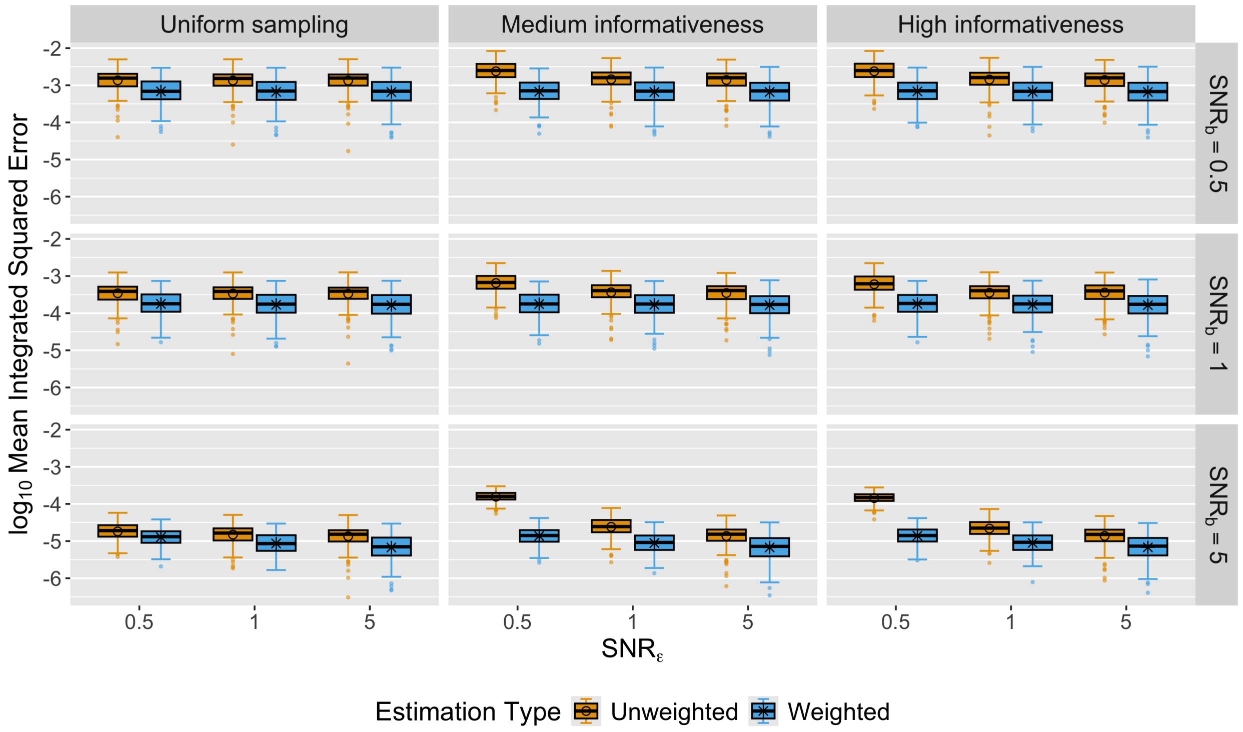


**Fig. S1.** MISE for functional intercept. $I_n$ and $L$ are fixed at 100 and 50, respectively, and there is both strata scaling and strata/PSU random effects

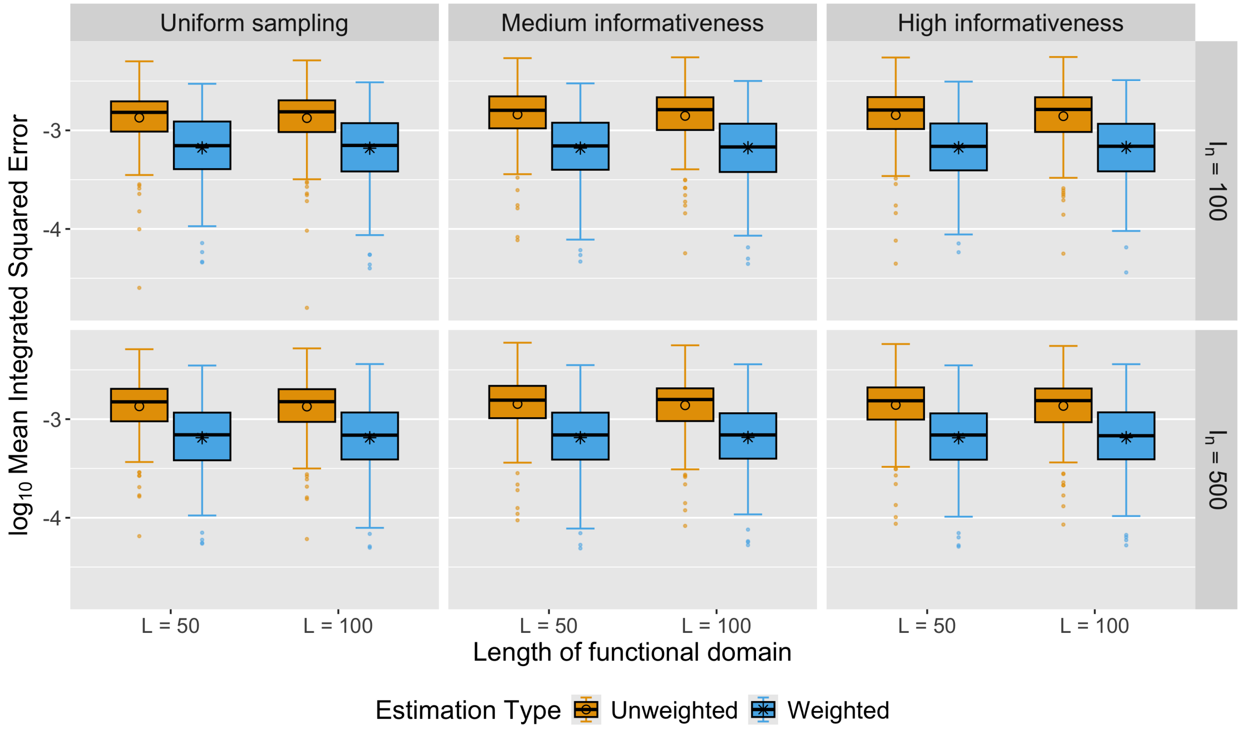


**Fig. S2.** MISE for functional intercept. Signal to noise ratio is fixed at 1, relative importance of fixed effects is fixed at 0.5, and there is both strata scaling and strata/PSU random effects

### *A.2. Signal-to-noise parameters and random effects strength*

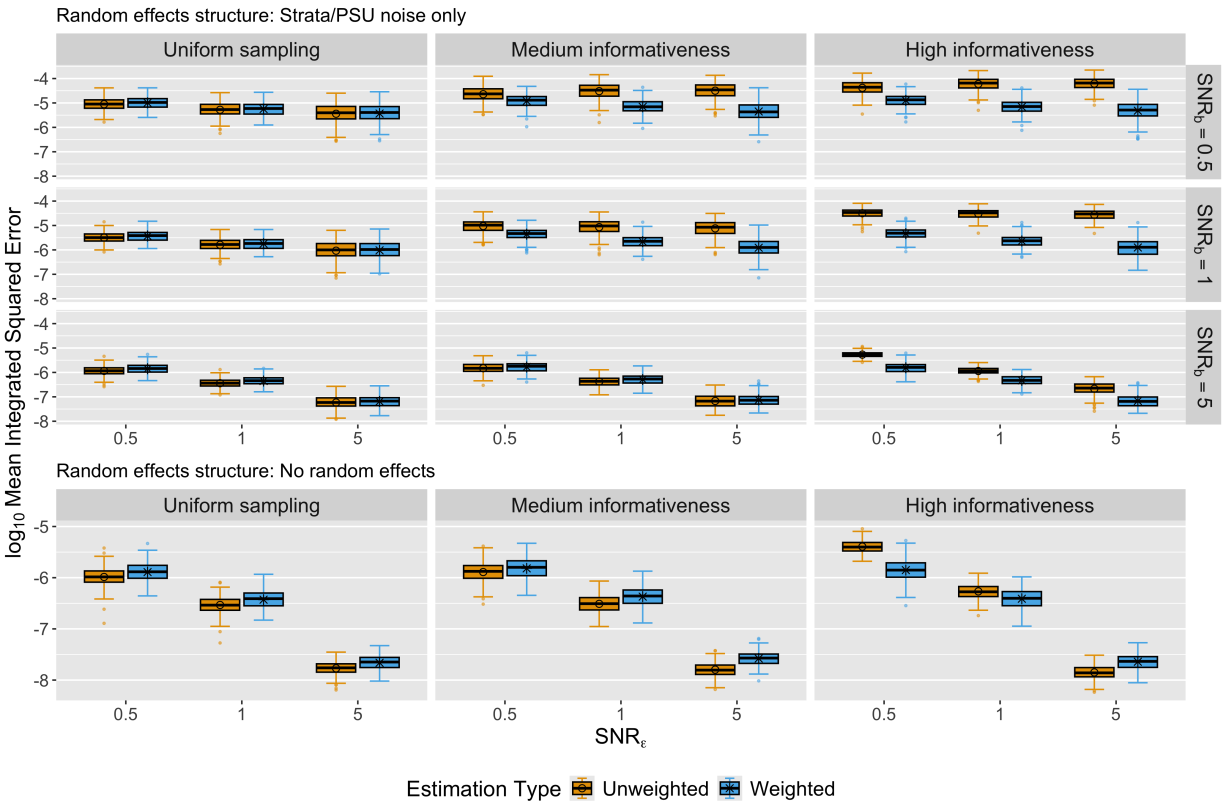


**Fig. S3.** MISE for functional coefficient $X$. Top: log MISE for varied signal-to-noise parameters and sampling schemes, with strata/PSU noise only for the random effects structure. Bottom: log MISE for varied sampling schemes and signal to noise ratios with no random effects.

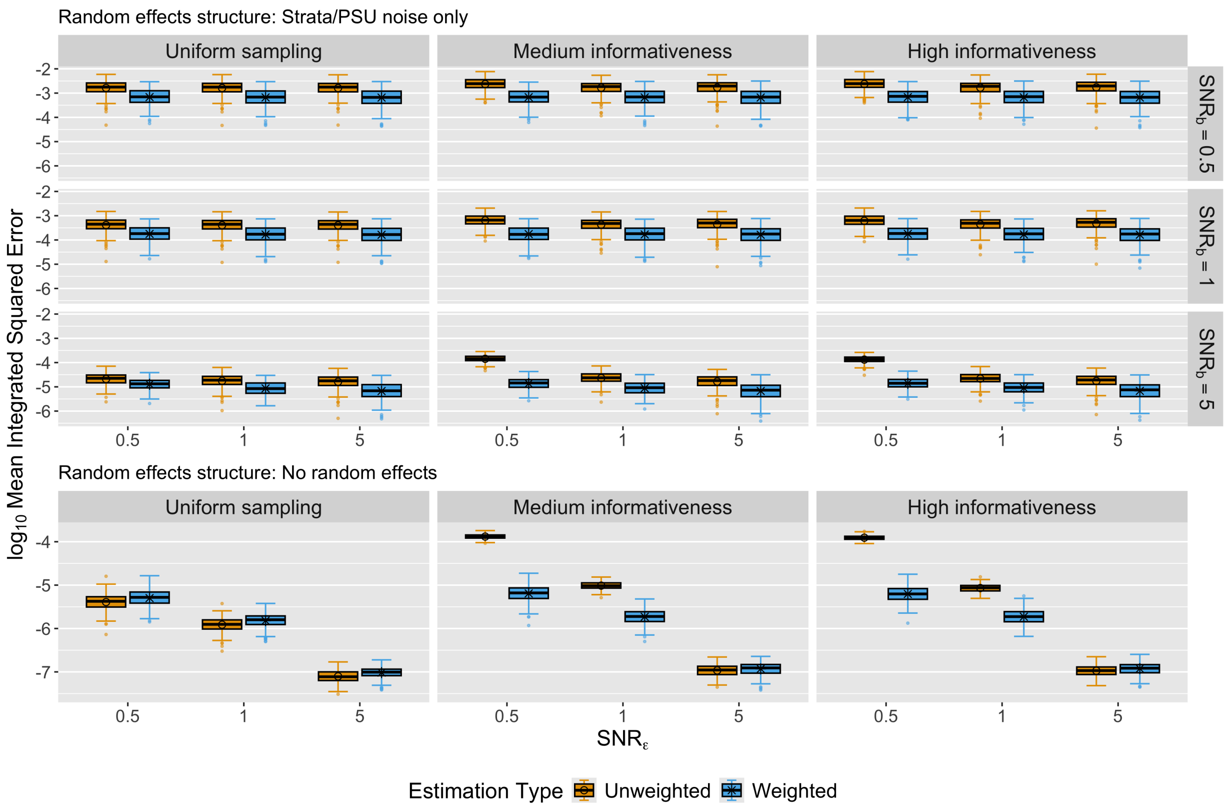


**Fig. S4.** MISE for functional intercept. Top: log MISE for varied signal-to-noise parameters and sampling schemes, with strata/PSU noise only for the random effects structure. Bottom: log MISE for varied sampling schemes and signal to noise ratios with no random effects.

***A.3. Sample size and functional domain length***

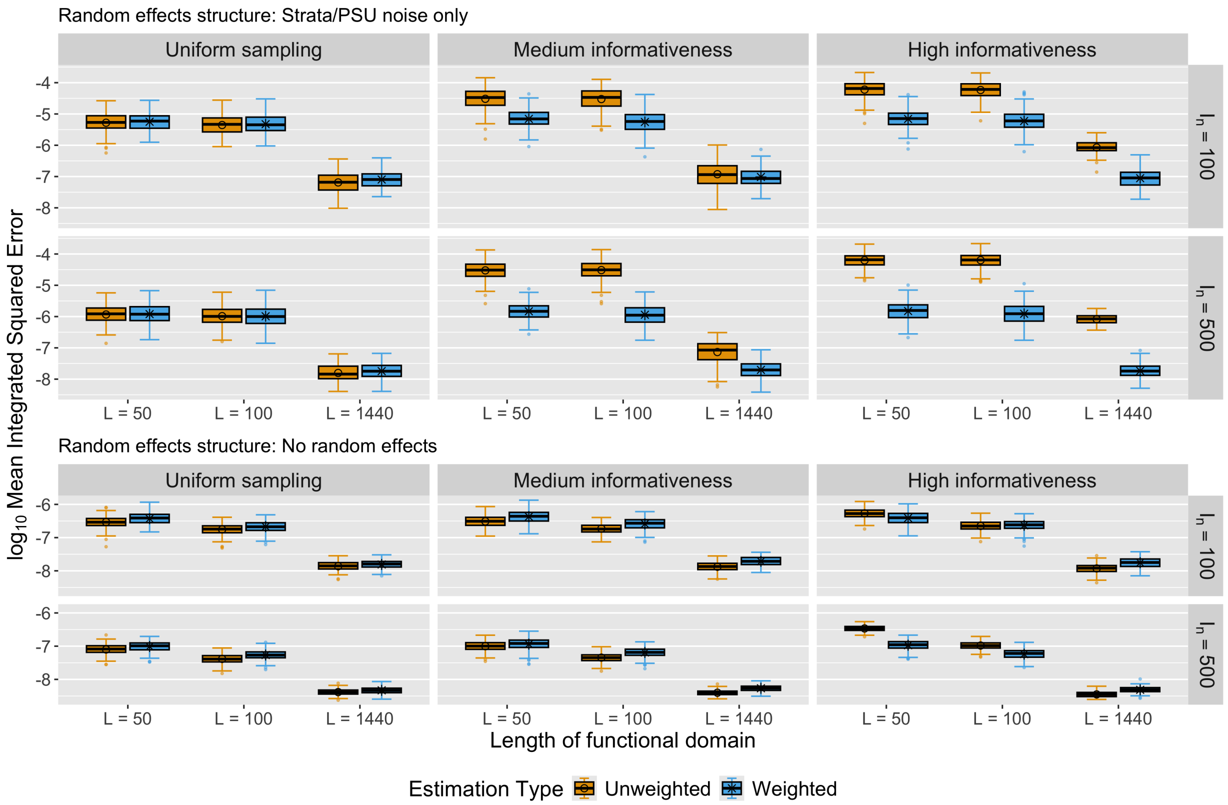


**Fig. S5.** MISE for functional coefficient $X$. Top: log MISE for varied sample sizes and functional domain length, with strata/PSU noise only for the random effects structure. Bottom: log MISE for varied sample sizes and functional domain length with no random effects.

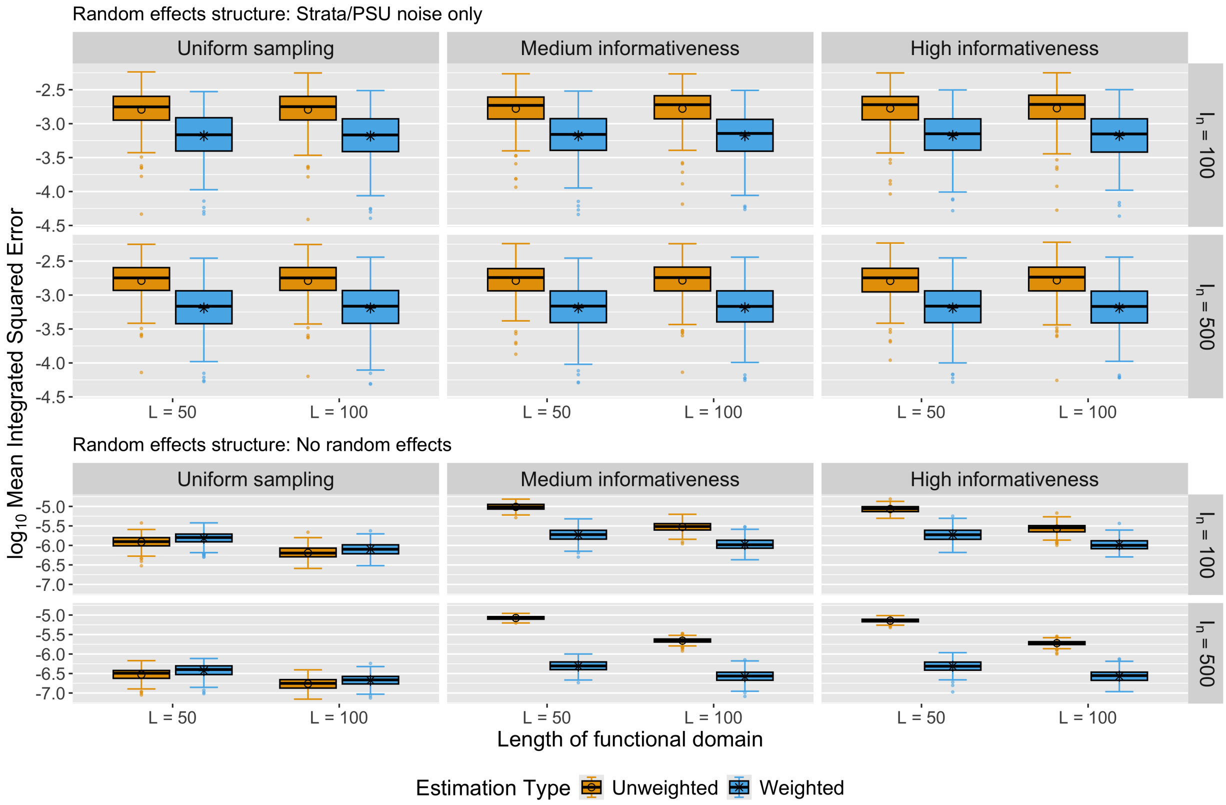


**Fig. S6.** MISE for functional intercept. Top: log MISE for varied sample sizes and functional domain length, with strata/PSU noise only for the random effects structure. Bottom: log MISE for varied sample sizes and functional domain length with no random effects.

## B. Non-Gaussian data

### *B.1. Random effects strength*

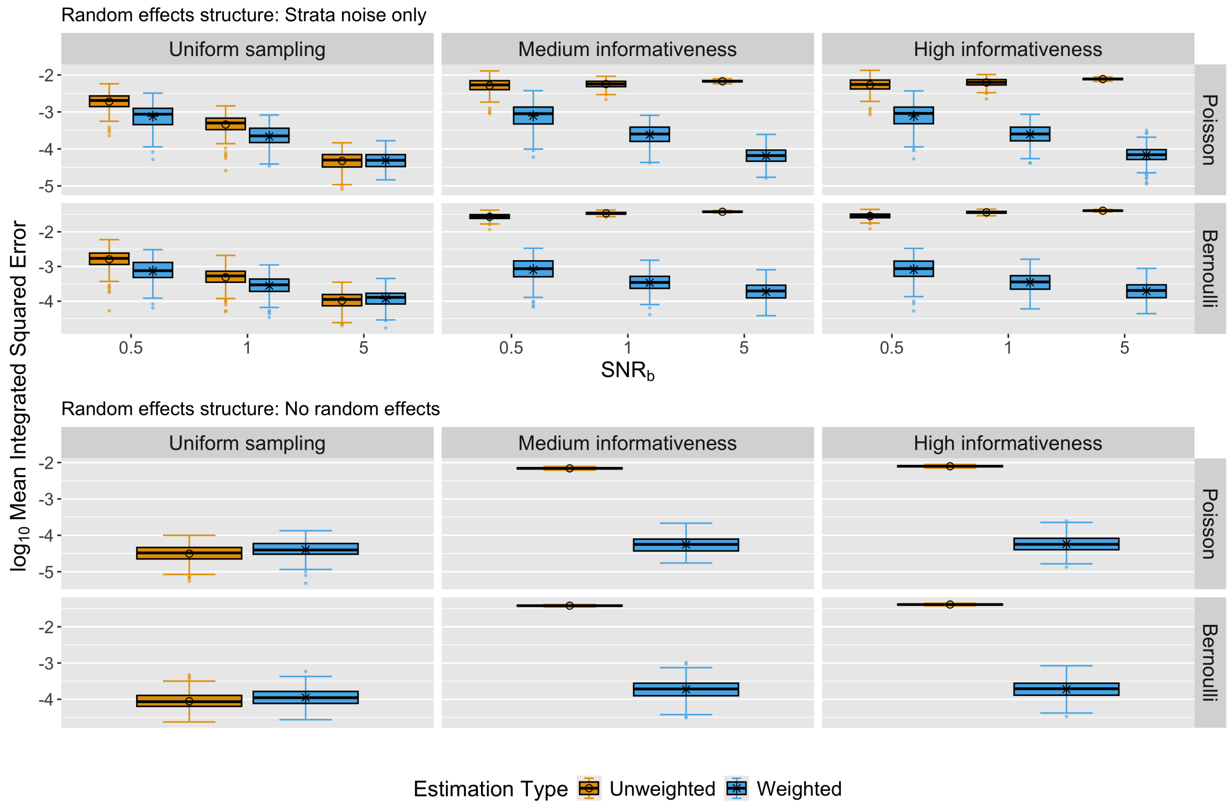


**Fig. S7.** MISE for functional coefficient $X$. Top: log MISE for varied strength of random effects, with strata/PSU noise only for the random effects structure. Bottom: log MISE with no random effects.

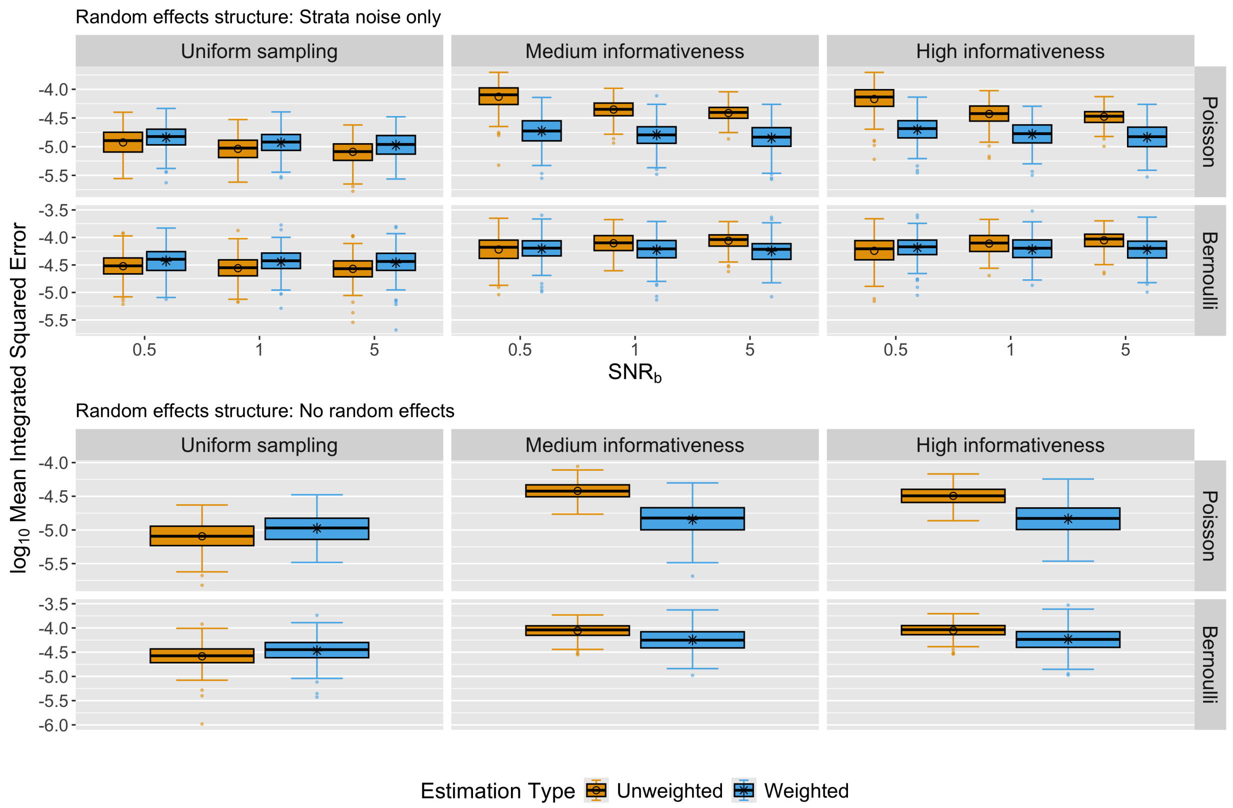


**Fig. S8.** MISE for functional intercept. Top: log MISE for varied strength of random effects, with strata/PSU noise only for the random effects structure. Bottom: log MISE with no random effects.

### *B.2. Sample size parameters and functional domain length*

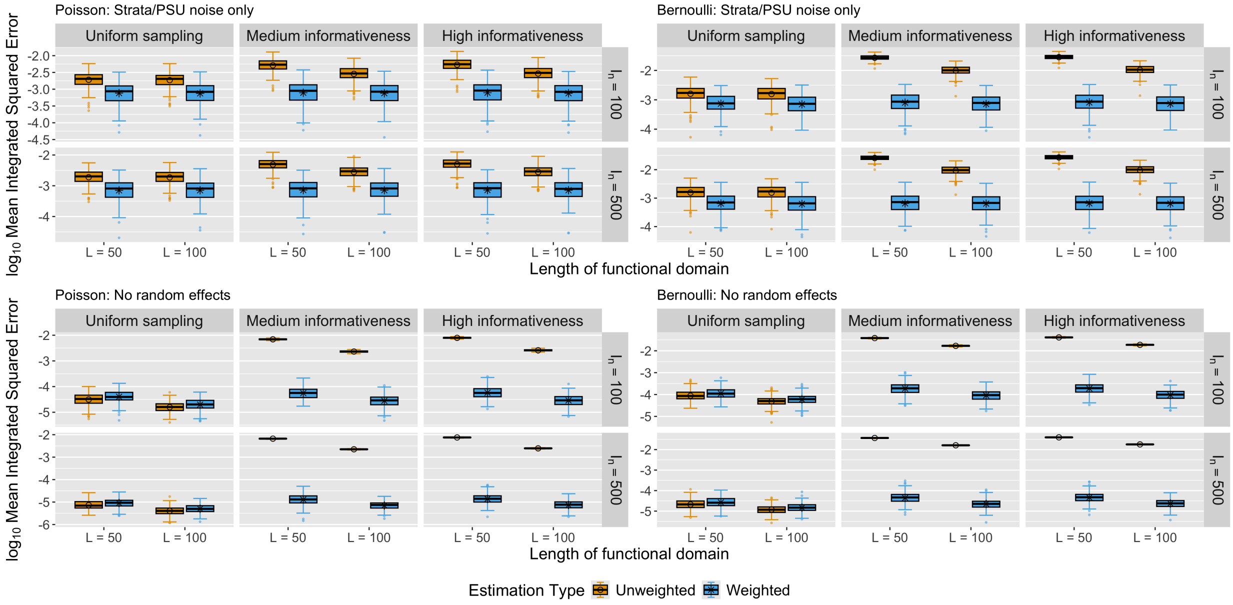


**Fig. S9.** MISE for functional coefficient $X$. Top: log MISE for varied sample size and functional domain length, with strata/PSU noise only, for Poisson (left) and Bernoulli (right). Bottom: log MISE for varied sample size and functional domain length, with no random effects, for Poisson (left) and Bernoulli (right).

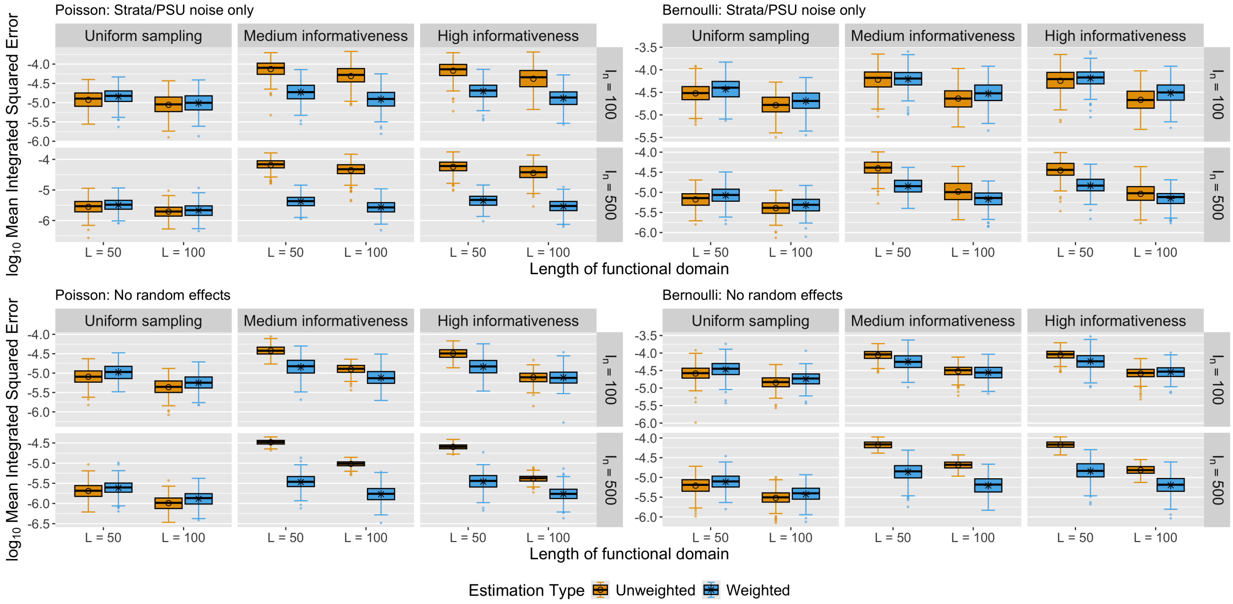


**Fig. S10.** MISE for functional intercept. Top: log MISE for varied sample size and functional domain length, with strata/PSU noise only, for Poisson (left) and Bernoulli (right). Bottom: log MISE for varied sample size and functional domain length, with no random effects, for Poisson (left) and Bernoulli (right)

## 2. POINTWISE COVERAGE PROBABILITIES

| Model | Uniform sampling | | Medium informativeness | | High informativeness | |
|---|---|---|---|---|---|---|
| | Poisson | Bernoulli | Poisson | Bernoulli | Poisson | Bernoulli |
| Unweighted | 0.97 | 0.95 | 0.54 | 0.87 | 0.60 | 0.88 |
| Weighted | 0.96 | 0.94 | 0.95 | 0.90 | 0.94 | 0.89 |
| BRR | 0.95 | 0.94 | 0.94 | 0.94 | 0.95 | 0.94 |
| RWYB | 0.96 | 0.94 | 0.95 | 0.94 | 0.95 | 0.94 |
| Model | No random effects | | Noise only | | Scaling & noise | |
| | Poisson | Bernoulli | Poisson | Bernoulli | Poisson | Bernoulli |
| Unweighted | 0.530 | 0.70 | 0.41 | 0.83 | 0.54 | 0.87 |
| Weighted | 0.94 | 0.88 | 0.94 | 0.90 | 0.95 | 0.90 |
| BRR | 0.95 | 0.94 | 0.95 | 0.94 | 0.94 | 0.94 |
| RWYB | 0.95 | 0.94 | 0.95 | 0.94 | 0.95 | 0.94 |
| Model | $\text{SNR}_b = 0.5$ | | $\text{SNR}_b = 1$ | | $\text{SNR}_b = 5$ | |
| | Poisson | Bernoulli | Poisson | Bernoulli | Poisson | Bernoulli |
| Unweighted | 0.54 | 0.87 | 0.58 | 0.78 | 0.534 | 0.70 |
| Weighted | 0.95 | 0.90 | 0.94 | 0.88 | 0.94 | 0.88 |
| BRR | 0.94 | 0.94 | 0.94 | 0.93 | 0.95 | 0.94 |
| RWYB | 0.95 | 0.94 | 0.95 | 0.94 | 0.95 | 0.94 |
| Model | $I_n = 100$ | | $I_n = 500$ | | | |
| | Poisson | Bernoulli | Poisson | Bernoulli | | |
| Unweighted | 0.54 | 0.87 | 0.18 | 0.57 | | |
| Weighted | 0.95 | 0.90 | 0.95 | 0.91 | | |
| BRR | 0.94 | 0.94 | 0.95 | 0.93 | | |
| RWYB | 0.95 | 0.94 | 0.95 | 0.93 | | |
| Model | $L = 50$ | | $L = 100$ | | | |
| | Poisson | Bernoulli | Poisson | Bernoulli | | |
| Unweighted | 0.54 | 0.87 | 0.61 | 0.94 | | |
| Weighted | 0.95 | 0.90 | 0.94 | 0.93 | | |
| BRR | 0.94 | 0.94 | 0.94 | 0.94 | | |
| RWYB | 0.95 | 0.94 | 0.94 | 0.95 | | |

**Table S1.** Non-Gaussian data: empirical coverage probability for the functional intercept of 95% pointwise coverage bands with each method from 200 simulations. The baseline setting is $I_n = 100, L = 50, \text{SNR}_b = 0.5$, medium informativeness, and strata/PSU scaling and noise. All other parameters are fixed at their baseline values when another parameter is changed.

## 3. JOINT COVERAGE PROBABILITIES

### A. Gaussian data

| Model | Uniform sampling | | Medium informativeness | | High informativeness | |
|---|---|---|---|---|---|---|
| | Intercept | $X$ | Intercept | $X$ | Intercept | $X$ |
| Unweighted | 0.01 | 0.95 | 0.00 | 0.10 | 0.01 | 0.01 |
| Weighted | 0.01 | 0.94 | 0.01 | 0.90 | 0.00 | 0.89 |
| BRR | 0.92 | 0.93 | 0.92 | 0.91 | 0.92 | 0.89 |
| RWYB | 0.92 | 0.94 | 0.92 | 0.93 | 0.93 | 0.92 |
| Model | No random effects | | Noise only | | Scaling & noise | |
| | Intercept | $X$ | Intercept | $X$ | Intercept | $X$ |
| Unweighted | 0.01 | 0.96 | 0.00 | 0.24 | 0.00 | 0.10 |
| Weighted | 0.85 | 0.94 | 0.01 | 0.91 | 0.01 | 0.90 |
| BRR | 0.82 | 0.85 | 0.91 | 0.94 | 0.92 | 0.91 |
| RWYB | 0.81 | 0.88 | 0.93 | 0.94 | 0.92 | 0.93 |
| Model | $\text{SNR}_b = 0.5$ | | $\text{SNR}_b = 1$ | | $\text{SNR}_b = 5$ | |
| | Intercept | $X$ | Intercept | $X$ | Intercept | $X$ |
| Unweighted | 0.00 | 0.10 | 0.01 | 0.11 | 0.00 | 0.95 |
| Weighted | 0.01 | 0.90 | 0.01 | 0.92 | 0.14 | 0.91 |
| BRR | 0.92 | 0.91 | 0.91 | 0.93 | 0.89 | 0.85 |
| RWYB | 0.92 | 0.93 | 0.92 | 0.93 | 0.90 | 0.86 |
| Model | $\text{SNR}_\epsilon = 0.5$ | | $\text{SNR}_\epsilon = 1$ | | $\text{SNR}_\epsilon = 5$ | |
| | Intercept | $X$ | Intercept | $X$ | Intercept | $X$ |
| Unweighted | 0.00 | 0.40 | 0.00 | 0.10 | 0.00 | 0.04 |
| Weighted | 0.02 | 0.93 | 0.01 | 0.90 | 0.00 | 0.91 |
| BRR | 0.92 | 0.92 | 0.92 | 0.91 | 0.94 | 0.91 |
| RWYB | 0.93 | 0.92 | 0.92 | 0.93 | 0.93 | 0.92 |
| Model | $I_n = 100$ | | $I_n = 500$ | | | |
| | Intercept | $X$ | Intercept | $X$ | | |
| Unweighted | 0.00 | 0.10 | 0.00 | 0.00 | | |
| Weighted | 0.01 | 0.90 | 0.00 | 0.91 | | |
| BRR | 0.92 | 0.91 | 0.92 | 0.94 | | |
| RWYB | 0.92 | 0.93 | 0.90 | 0.94 | | |
| Model | $L = 50$ | | $L = 100$ | | $L = 1440$ | |
| | Intercept | $X$ | Intercept | $X$ | Intercept | $X$ |
| Unweighted | 0.00 | 0.10 | 0.01 | 0.09 | | 0.82 |
| Weighted | 0.01 | 0.90 | 0.00 | 0.91 | | 0.95 |
| BRR | 0.92 | 0.91 | 0.90 | 0.91 | | 0.89 |
| RWYB | 0.92 | 0.93 | 0.92 | 0.92 | | 0.87 |

**Table S2.** Gaussian data: empirical coverage probability of 95% joint coverage bands with each method from 200 simulations. The baseline setting is $I_n = 100, L = 50, \text{SNR}_b = 0.5, \text{SNR}_\epsilon = 1$, medium informativeness, and strata/PSU scaling and noise. All other parameters are fixed at their baseline values when another parameter is changed.

## B. Non-Gaussian data

### *B.1. Functional coefficient*

| Model | Uniform sampling | | Medium informativeness | | High informativeness | |
|---|---|---|---|---|---|---|
| | Poisson | Bernoulli | Poisson | Bernoulli | Poisson | Bernoulli |
| Unweighted | 0.01 | 0.03 | 0.00 | 0.00 | 0.00 | 0.00 |
| Weighted | 0.04 | 0.15 | 0.04 | 0.17 | 0.04 | 0.15 |
| BRR | 0.85 | 0.85 | 0.81 | 0.85 | 0.81 | 0.86 |
| RWYB | 0.87 | 0.87 | 0.81 | 0.85 | 0.81 | 0.87 |
| **Model** | **No random effects** | | **Noise only** | | **Scaling & noise** | |
| | Poisson | Bernoulli | Poisson | Bernoulli | Poisson | Bernoulli |
| Unweighted | 0.00 | 0.00 | 0.00 | 0.00 | 0.00 | 0.00 |
| Weighted | 0.84 | 0.77 | 0.04 | 0.15 | 0.04 | 0.17 |
| BRR | 0.92 | 0.89 | 0.82 | 0.85 | 0.81 | 0.85 |
| RWYB | 0.93 | 0.91 | 0.82 | 0.85 | 0.81 | 0.85 |
| **Model** | $\text{SNR}_b = 0.5$ | | $\text{SNR}_b = 1$ | | $\text{SNR}_b = 5$ | |
| | Poisson | Bernoulli | Poisson | Bernoulli | Poisson | Bernoulli |
| Unweighted | 0.00 | 0.00 | 0.000 | 0.00 | 0.00 | 0.00 |
| Weighted | 0.04 | 0.17 | 0.18 | 0.42 | 0.75 | 0.73 |
| BRR | 0.81 | 0.85 | 0.84 | 0.88 | 0.89 | 0.91 |
| RWYB | 0.81 | 0.85 | 0.82 | 0.90 | 0.90 | 0.91 |
| **Model** | $I_n = 100$ | | $I_n = 500$ | | | |
| | Poisson | Bernoulli | Poisson | Bernoulli | | |
| Unweighted | 0.00 | 0.00 | 0.00 | 0.00 | | |
| Weighted | 0.04 | 0.17 | 0.01 | 0.02 | | |
| BRR | 0.81 | 0.85 | 0.86 | 0.90 | | |
| RWYB | 0.81 | 0.85 | 0.85 | 0.88 | | |
| **Model** | $L = 50$ | | $L = 100$ | | | |
| | Poisson | Bernoulli | Poisson | Bernoulli | | |
| Unweighted | 0.00 | 0.00 | 0.00 | 0.00 | | |
| Weighted | 0.04 | 0.17 | 0.01 | 0.08 | | |
| BRR | 0.81 | 0.85 | 0.88 | 0.89 | | |
| RWYB | 0.81 | 0.85 | 0.87 | 0.90 | | |

**Table S3.** Non-Gaussian data: empirical coverage probability for the functional coefficient of 95% joint coverage bands with each method from 200 simulations. The baseline setting is $I_n = 100, L = 50, \text{SNR}_b = 0.5$, medium informativeness, and strata/PSU scaling and noise. All other parameters are fixed at their baseline values when another parameter is changed.

*B.2. Functional intercept*

| Model | Uniform sampling | | Medium informativeness | | High informativeness | |
|---|---|---|---|---|---|---|
| | Poisson | Bernoulli | Poisson | Bernoulli | Poisson | Bernoulli |
| Unweighted | 0.95 | 0.94 | 0.26 | 0.82 | 0.34 | 0.82 |
| Weighted | 0.95 | 0.91 | 0.92 | 0.79 | 0.91 | 0.76 |
| BRR | 0.92 | 0.85 | 0.93 | 0.88 | 0.93 | 0.92 |
| RWYB | 0.93 | 0.89 | 0.95 | 0.88 | 0.92 | 0.89 |
| Model | No random effects | | Noise only | | Scaling & noise | |
| | Poisson | Bernoulli | Poisson | Bernoulli | Poisson | Bernoulli |
| Unweighted | 0.08 | 0.47 | 0.12 | 0.73 | 0.26 | 0.82 |
| Weighted | 0.91 | 0.66 | 0.90 | 0.79 | 0.92 | 0.79 |
| BRR | 0.88 | 0.86 | 0.92 | 0.91 | 0.93 | 0.88 |
| RWYB | 0.89 | 0.86 | 0.93 | 0.91 | 0.95 | 0.88 |
| Model | $\text{SNR}_b = 0.5$ | | $\text{SNR}_b = 1$ | | $\text{SNR}_b = 5$ | |
| | Poisson | Bernoulli | Poisson | Bernoulli | Poisson | Bernoulli |
| Unweighted | 0.26 | 0.82 | 0.16 | 0.63 | 0.09 | 0.52 |
| Weighted | 0.92 | 0.79 | 0.87 | 0.70 | 0.90 | 0.68 |
| BRR | 0.93 | 0.88 | 0.89 | 0.85 | 0.87 | 0.89 |
| RWYB | 0.95 | 0.88 | 0.90 | 0.88 | 0.90 | 0.90 |
| Model | $I_n = 100$ | | $I_n = 500$ | | | |
| | Poisson | Bernoulli | Poisson | Bernoulli | | |
| Unweighted | 0.26 | 0.82 | 0.01 | 0.27 | | |
| Weighted | 0.92 | 0.79 | 0.92 | 0.84 | | |
| BRR | 0.93 | 0.88 | 0.89 | 0.87 | | |
| RWYB | 0.95 | 0.88 | 0.90 | 0.87 | | |
| Model | $L = 50$ | | $L = 100$ | | | |
| | Poisson | Bernoulli | Poisson | Bernoulli | | |
| Unweighted | 0.26 | 0.82 | 0.31 | 0.95 | | |
| Weighted | 0.92 | 0.79 | 0.93 | 0.88 | | |
| BRR | 0.93 | 0.88 | 0.92 | 0.87 | | |
| RWYB | 0.95 | 0.88 | 0.94 | 0.88 | | |

**Table S4.** Non-Gaussian data: empirical coverage probability for the functional intercept of 95% joint coverage bands with each method from 200 simulations. The baseline setting is $I_n = 100, L = 50, \text{SNR}_b = 0.5$, medium informativeness, and strata/PSU scaling and noise. All other parameters are fixed at their baseline values when another parameter is changed.

## 4. QUANTIFYING WITHIN/BETWEEN STRATA AND PSU VARIABILITY

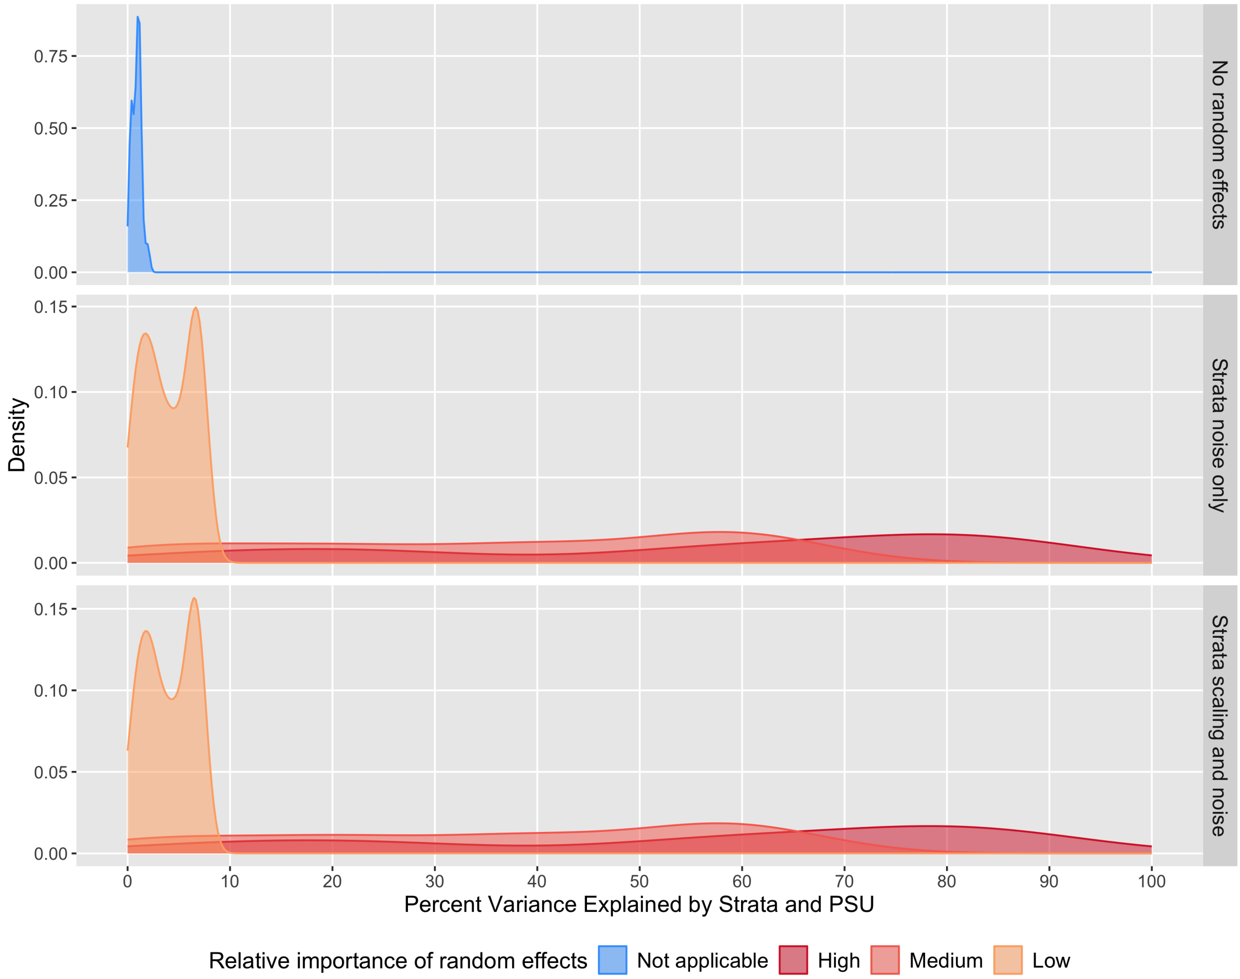


**Fig. S11.** Distribution of percent variance explained by strata and PSU, colored by relative importance of random effects and faceted by random effects structure. High relative importance of random effects means $\text{SNR}_b = 0.5$, medium means $\text{SNR}_b = 1$, and low means $\text{SNR}_b = 0.5$. We see that higher importance of random effects corresponds to more variance explained by strata/PSU.

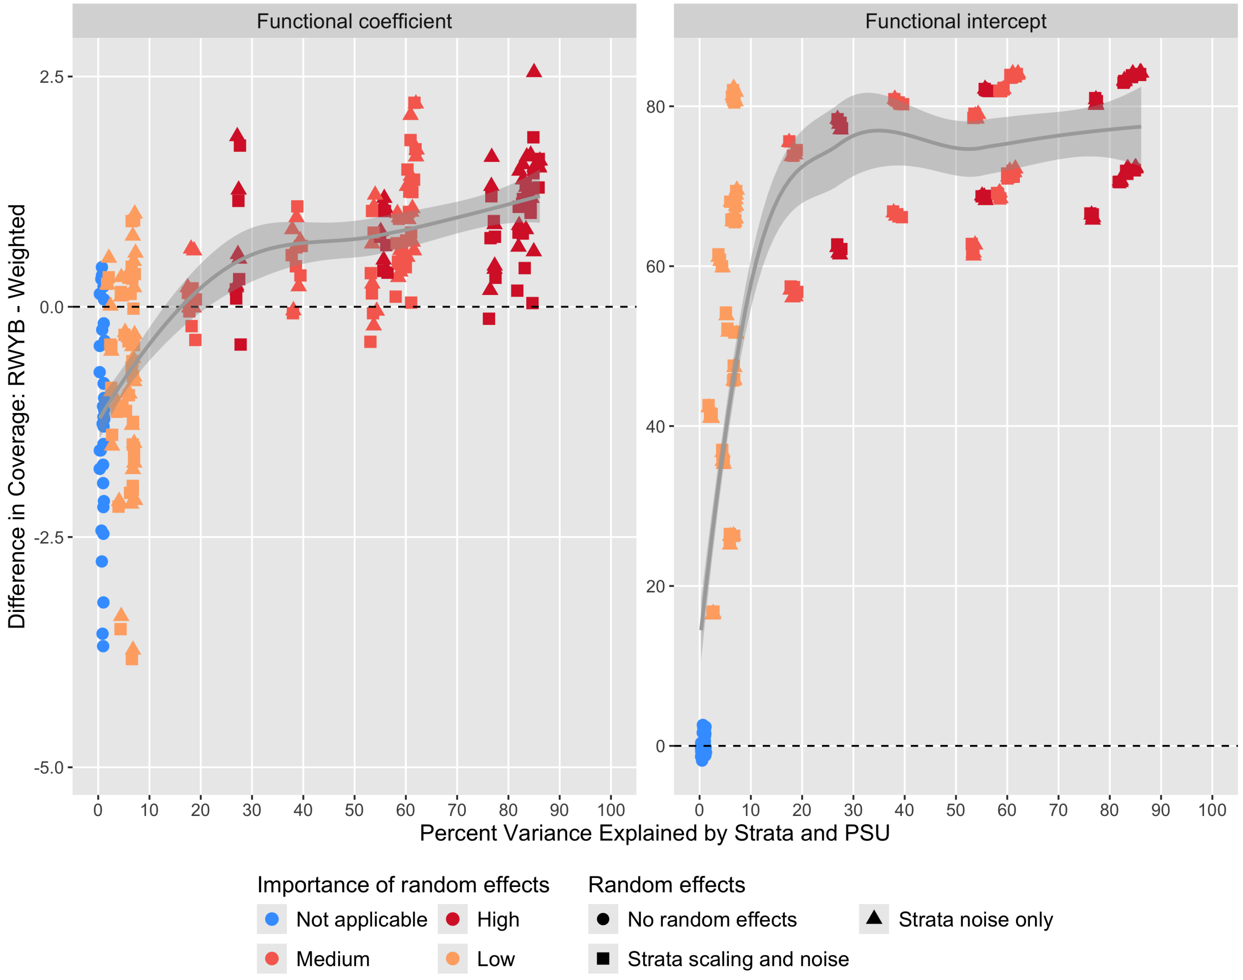


**Fig. S12.** Difference between RWYB coverage and weighted CI coverage (y-axis) vs. % variability explained by strata/PSU (x-axis, for functional coefficient (left panel) and functional intercept (right panel).

## 5. NHANES APPLICATION

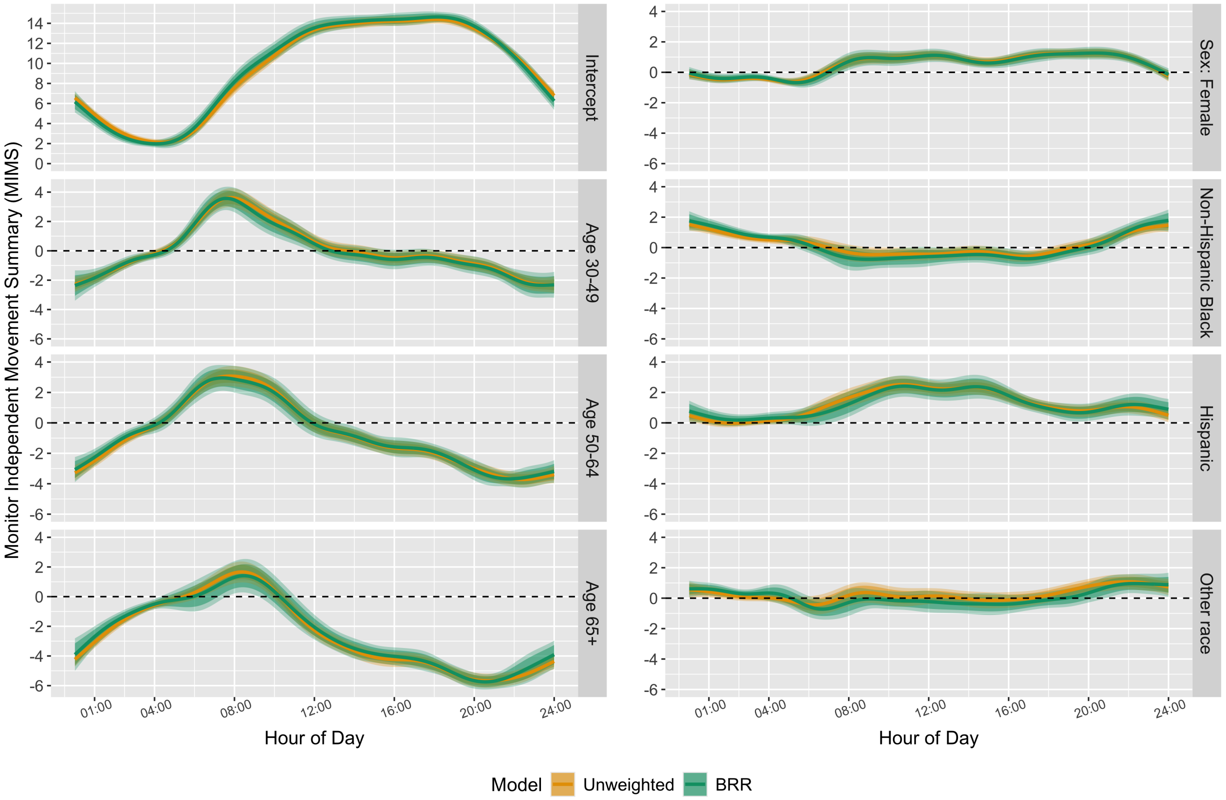


**Fig. S13.** Functional coefficient estimates for sex, age, and race. The reference categories are male, age 18-29, and white non-Hispanic race. The unweighted estimate is shown orange and the BRR estimate is shown in green. There is very small difference observed between the point estimates, but BRR confidence interval widths tend to be slightly larger.

| Coefficient | Agreement type | | | |
|---|---|---|---|---|
| | All 3 methods | BRR & Weighted | Weighed & Unweighted | BRR & Unweighted |
| Intercept | 100 | 100 | 100 | 100 |
| Age 30-49 | 95 | 98 | 96 | 97 |
| Age 50-64 | 96 | 97 | 99 | 96 |
| Age 65+ | 91 | 95 | 96 | 91 |
| Sex: Female | 96 | 99 | 98 | 97 |
| Non-Hispanic Black | 87 | 99 | 88 | 87 |
| Hispanic | 89 | 97 | 89 | 93 |
| Other race | 77 | 92 | 83 | 79 |

**Table S5.** Percent agreement in significance between each of the three methods (BRR, weighted, unweighted) in the NHANES application. 100% agreement means that in all 1440 locations across the functional domain, the confidence intervals from each method agreed (e.g. all included zero or all did not include zero.
